# Supplementary material for: Remedying Target-Domain Astigmatism for Cross-Domain Few-Shot Object Detection
Source: arXiv:2603.18541 source file (2026-03-19)
Supplement: Supplementary file 1 [file X_suppl.tex]

\clearpage
\setcounter{page}{1}
\maketitlesupplementary

%%%%%%%%%%%%%%%%%%%%%%%%%%%%%%%%%%%%%%%%%%%%%%%%%%%%%%%%%%%%%%%%%%%%%%%%%%%%%%%%%%%%
%%%%%%%%%%%%%%%%%%%%%%%%%%%%%%%%%%%%%%%%%%%%%%%%%%%%%%%%%%%%%%%%%%%%%%%%%%%%%%%%%%%%
\section{Cross-Domain Few-Shot Object Detection Problem Formulation}

Cross-Domain Few-Shot Object Detection (CD-FSOD) addresses the challenging scenario of adapting object detection models to novel target domains with limited labeled examples. Let $\mathcal{D}_S = \{(I_i^S, \mathcal{B}_i^S, \mathcal{C}_i^S)\}_{i=1}^{N_S}$ represent the source domain dataset with abundant labeled data (typically MS-COCO), where $I_i^S$ is an image, $\mathcal{B}_i^S = \{b_j^S\}_{j=1}^{n_i^S}$ denotes the set of bounding boxes, and $\mathcal{C}_i^S = \{c_j^S\}_{j=1}^{n_i^S}$ represents the corresponding class labels drawn from label space $\mathcal{C}_S$. Similarly, $\mathcal{D}_T = \{(I_i^T, \mathcal{B}_i^T, \mathcal{C}_i^T)\}_{i=1}^{N_T}$ represents the target domain dataset with class labels from $\mathcal{C}_T$.

The fundamental challenges in CD-FSOD stem from two factors: (1) \textbf{domain shift}, where the data distributions differ significantly between source and target domains ($P_S \neq P_T$); and (2) \textbf{limited supervision}, where only $K$ annotated examples per class (typically $K \in \{1,5,10\}$) are available in the target domain. During model development, we first train a detection model on the abundant source domain data $\mathcal{D}_S$, then adapt it to the target domain using the support set $\mathcal{S} = \{(I_i^T, \mathcal{B}_i^T, \mathcal{C}_i^T)\}_{i=1}^{N \times K}$ containing $K$ examples for each of the $N$ novel classes. The model is ultimately evaluated on the query set $\mathcal{Q}$ consisting of unseen target domain images.

Figure~\ref{fig:preliminaries} illustrates this setting, highlighting the substantial visual differences between the source domain (MS-COCO with diverse everyday objects) and target domains (specialized domains like clipart illustrations and satellite imagery). The cross-domain discrepancy manifests in various forms including changes in visual style, object appearance, background context, and imaging conditions. This setting presents unique opportunities to investigate knowledge transfer across visual domains while operating under extreme data constraints, requiring detection models that can effectively leverage source domain knowledge while adapting to the distinctive characteristics of the target domain with minimal supervision.

\begin{figure}[t]
    \centering
    \includegraphics[width=0.8\linewidth]{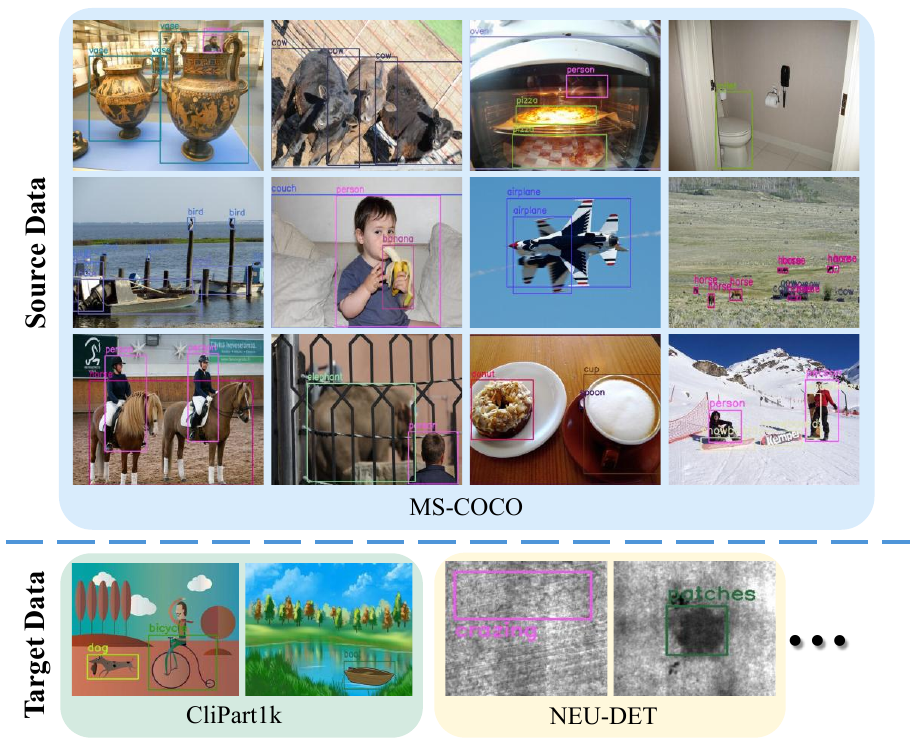}
    \caption{Illustration of the Cross-Domain Few-Shot Object Detection setting. The model is first trained on a labeled source domain (MS-COCO) with abundant data, then adapted to target domains (CliPart1k, NEU-DET, etc.) using only $K$ labeled examples per novel class. The figure demonstrates the significant visual domain gaps that models must overcome while learning from limited target domain supervision.}
    \label{fig:preliminaries}
\end{figure}

%%%%%%%%%%%%%%%%%%%%%%%%%%%%%%%%%%%%%%%%%%%%%%%%%%%%%%%%%%%%%%%%%%%%%%%%%%%%%%%%%%%%
%%%%%%%%%%%%%%%%%%%%%%%%%%%%%%%%%%%%%%%%%%%%%%%%%%%%%%%%%%%%%%%%%%%%%%%%%%%%%%%%%%%%
% \section{Dataset Visualization}

\section{Target Domain Datasets}

\textbf{ArTaxOr:} This arthropod detection dataset encompasses diverse biological classes including insects, spiders, crustaceans, and millipedes. The dataset presents significant challenges due to the morphological diversity across arthropod species, varying scales from microscopic to macroscopic organisms, and complex natural backgrounds that require fine-grained visual discrimination to distinguish between similar taxonomic groups, as shown in Figure~\ref{fig:artaxor_samples}.

\textbf{Clipart1k:} This dataset features cartoon-style abstractions that present a significant domain shift from natural photographs. The artistic rendering includes simplified geometric shapes, stylized color schemes, and abstract visual representations that challenge models trained on photorealistic images, as shown in Figure~\ref{fig:clipart1k_samples}.

\textbf{DIOR:} This remote sensing object detection dataset contains diverse annotated satellite imagery featuring objects such as airplanes, ships, and golf fields. The aerial perspective introduces unique challenges including large-scale variations, complex geographic backgrounds, and objects viewed from overhead angles that differ substantially from ground-level detection scenarios, as illustrated in Figure~\ref{fig:dior_samples}.

\textbf{DeepFish:} The underwater fish detection dataset introduces unique challenges including water distortion effects, varying lighting conditions, and complex aquatic environments. The marine setting creates substantial visual differences from terrestrial scenes with specialized underwater optics and marine backgrounds, as illustrated in Figure~\ref{fig:deepfish_samples}.

\textbf{NEU-DET:} This industrial dataset focuses on surface defect detection with subtle visual patterns and varying scales. The metallic surfaces and microscopic defects require fine-grained visual understanding and precise localization capabilities for quality control applications, as demonstrated in Figure~\ref{fig:neudet_samples}.

\textbf{UODD:} The underwater object detection dataset contains marine organisms in complex seafloor environments. The challenging conditions include varying water clarity, diverse lighting scenarios, and intricate backgrounds with coral reefs and marine vegetation that significantly differ from standard object detection scenarios, as shown in Figure~\ref{fig:uodd_samples}.

These datasets collectively demonstrate the diverse domain challenges that our center-periphery attention refinement framework addresses, validating the effectiveness of our approach across various types of domain shifts.

\begin{figure}[h]
\centering
\begin{subfigure}{0.2\textwidth}
    \includegraphics[width=\textwidth,height=3cm,keepaspectratio=false]{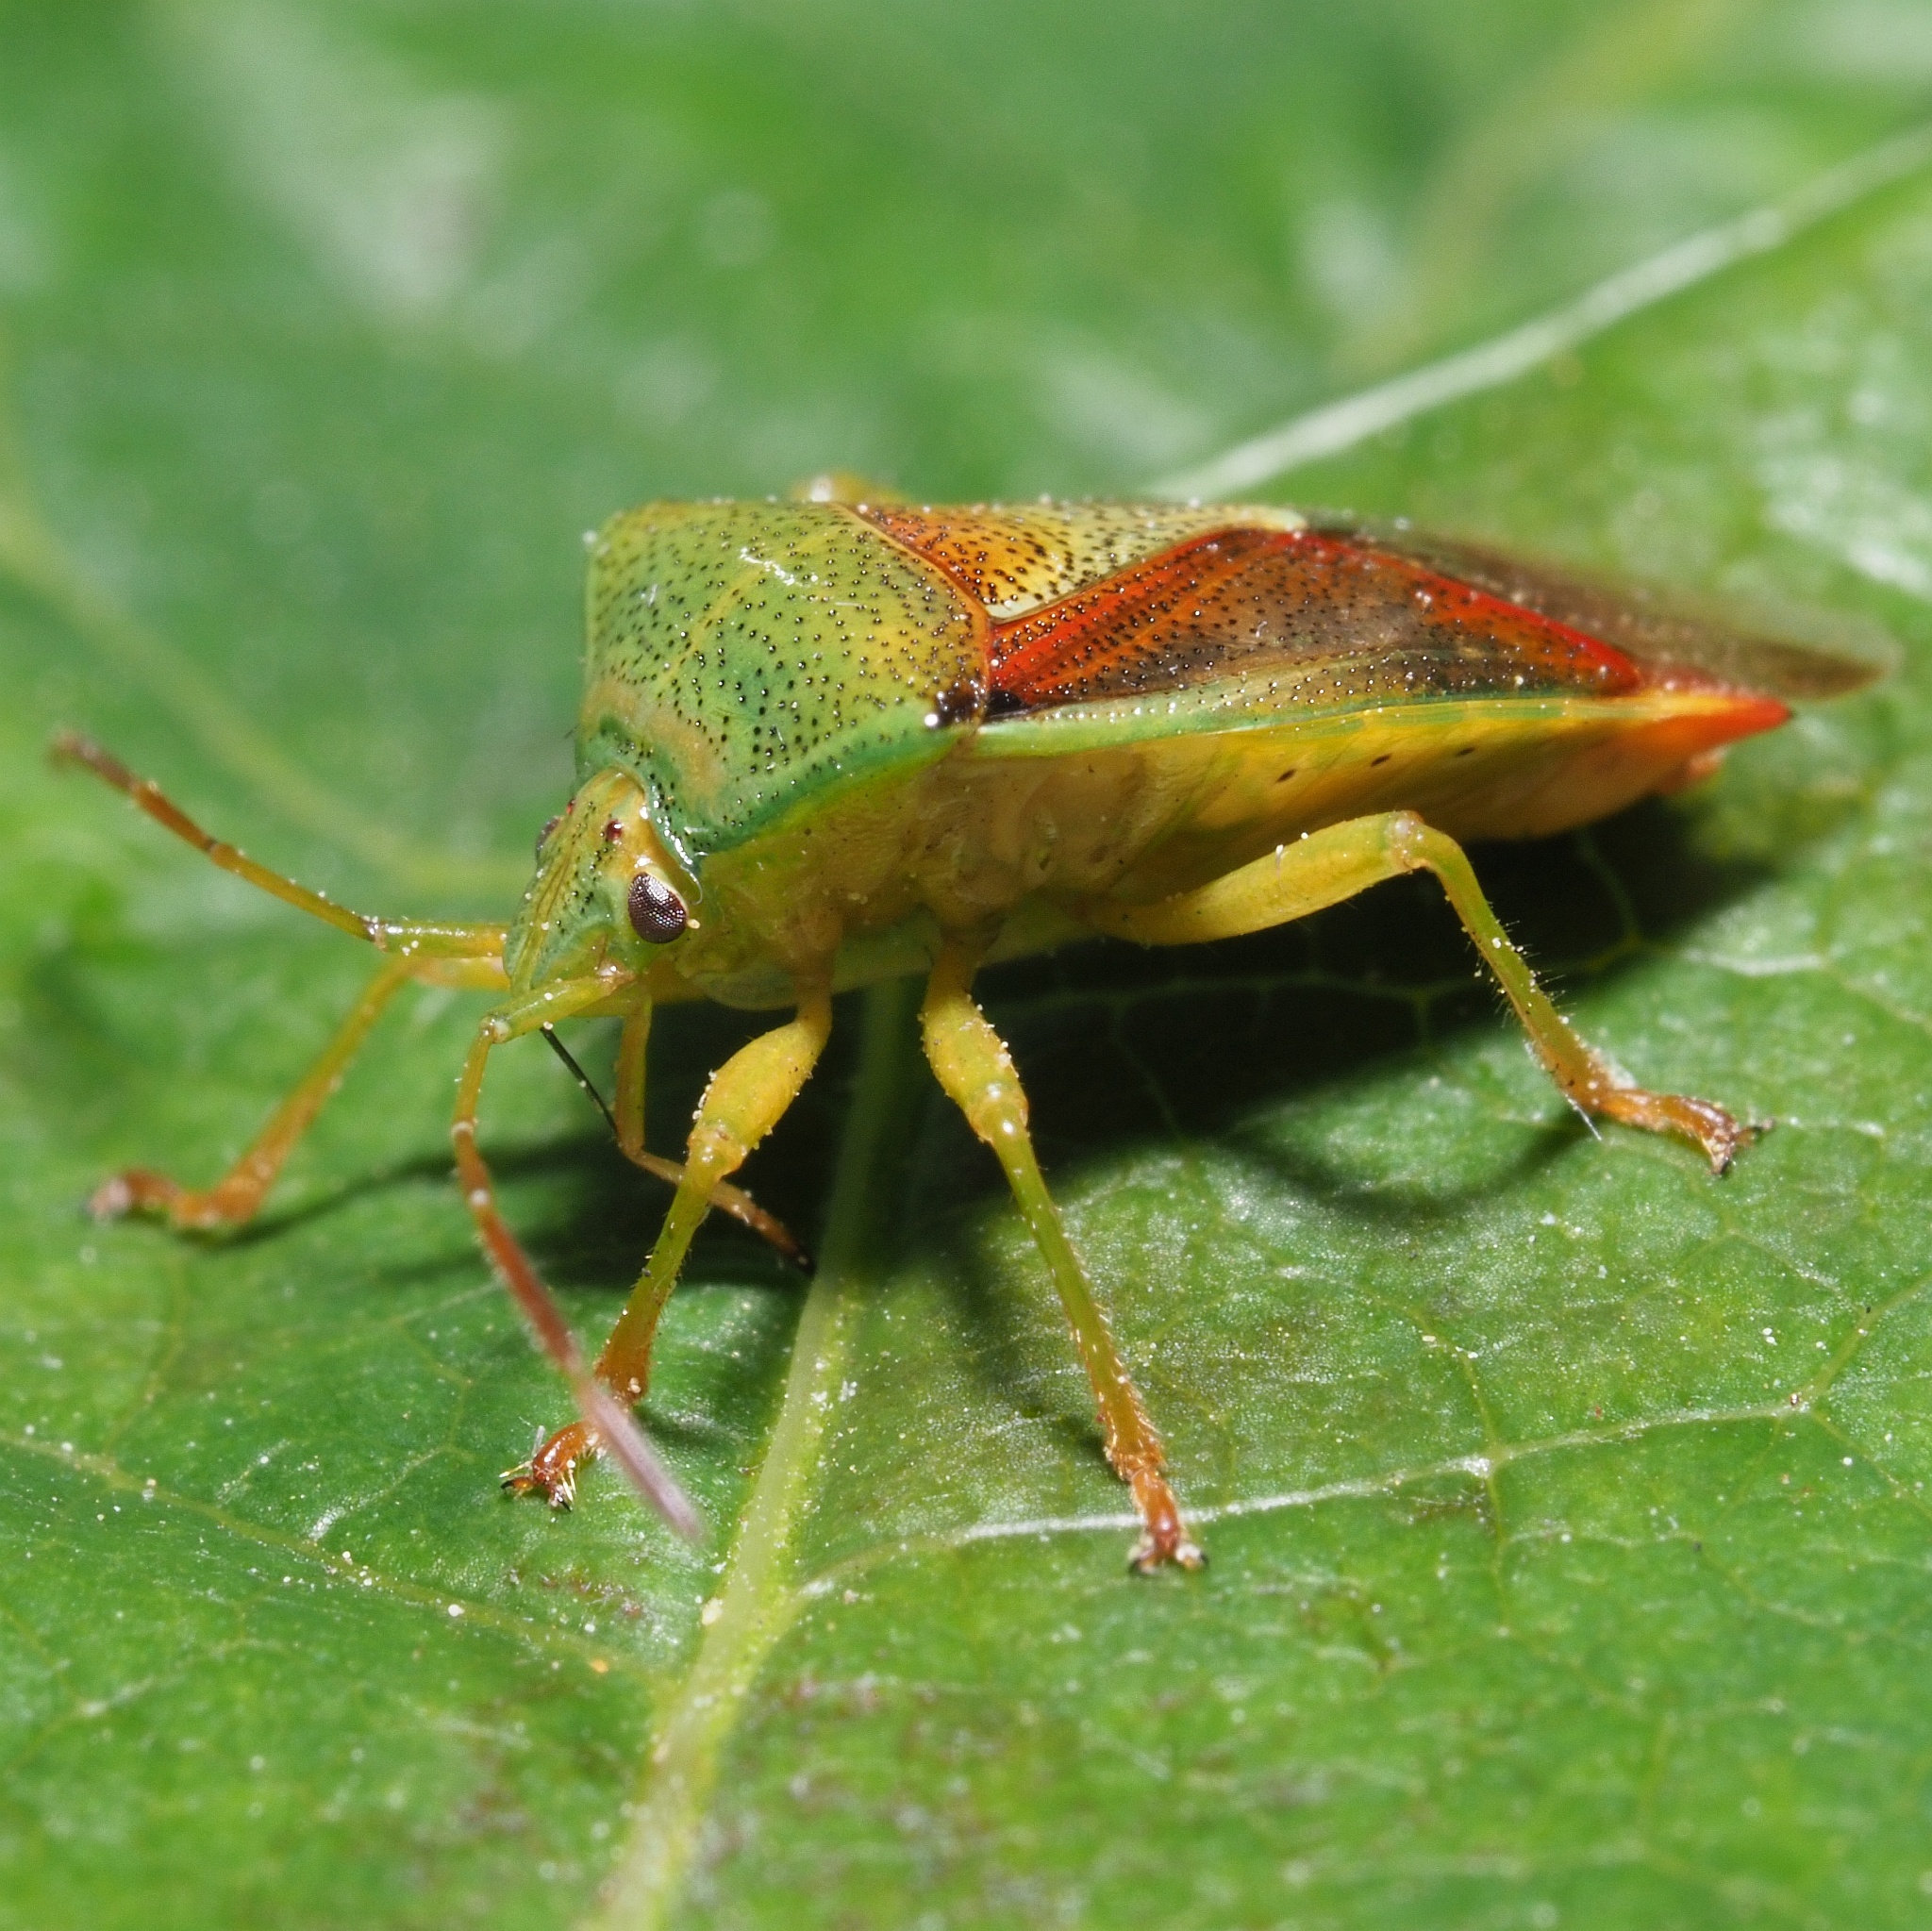}
\end{subfigure}%
\hspace{0.1cm}%
\begin{subfigure}{0.2\textwidth}
    \includegraphics[width=\textwidth,height=3cm,keepaspectratio=false]{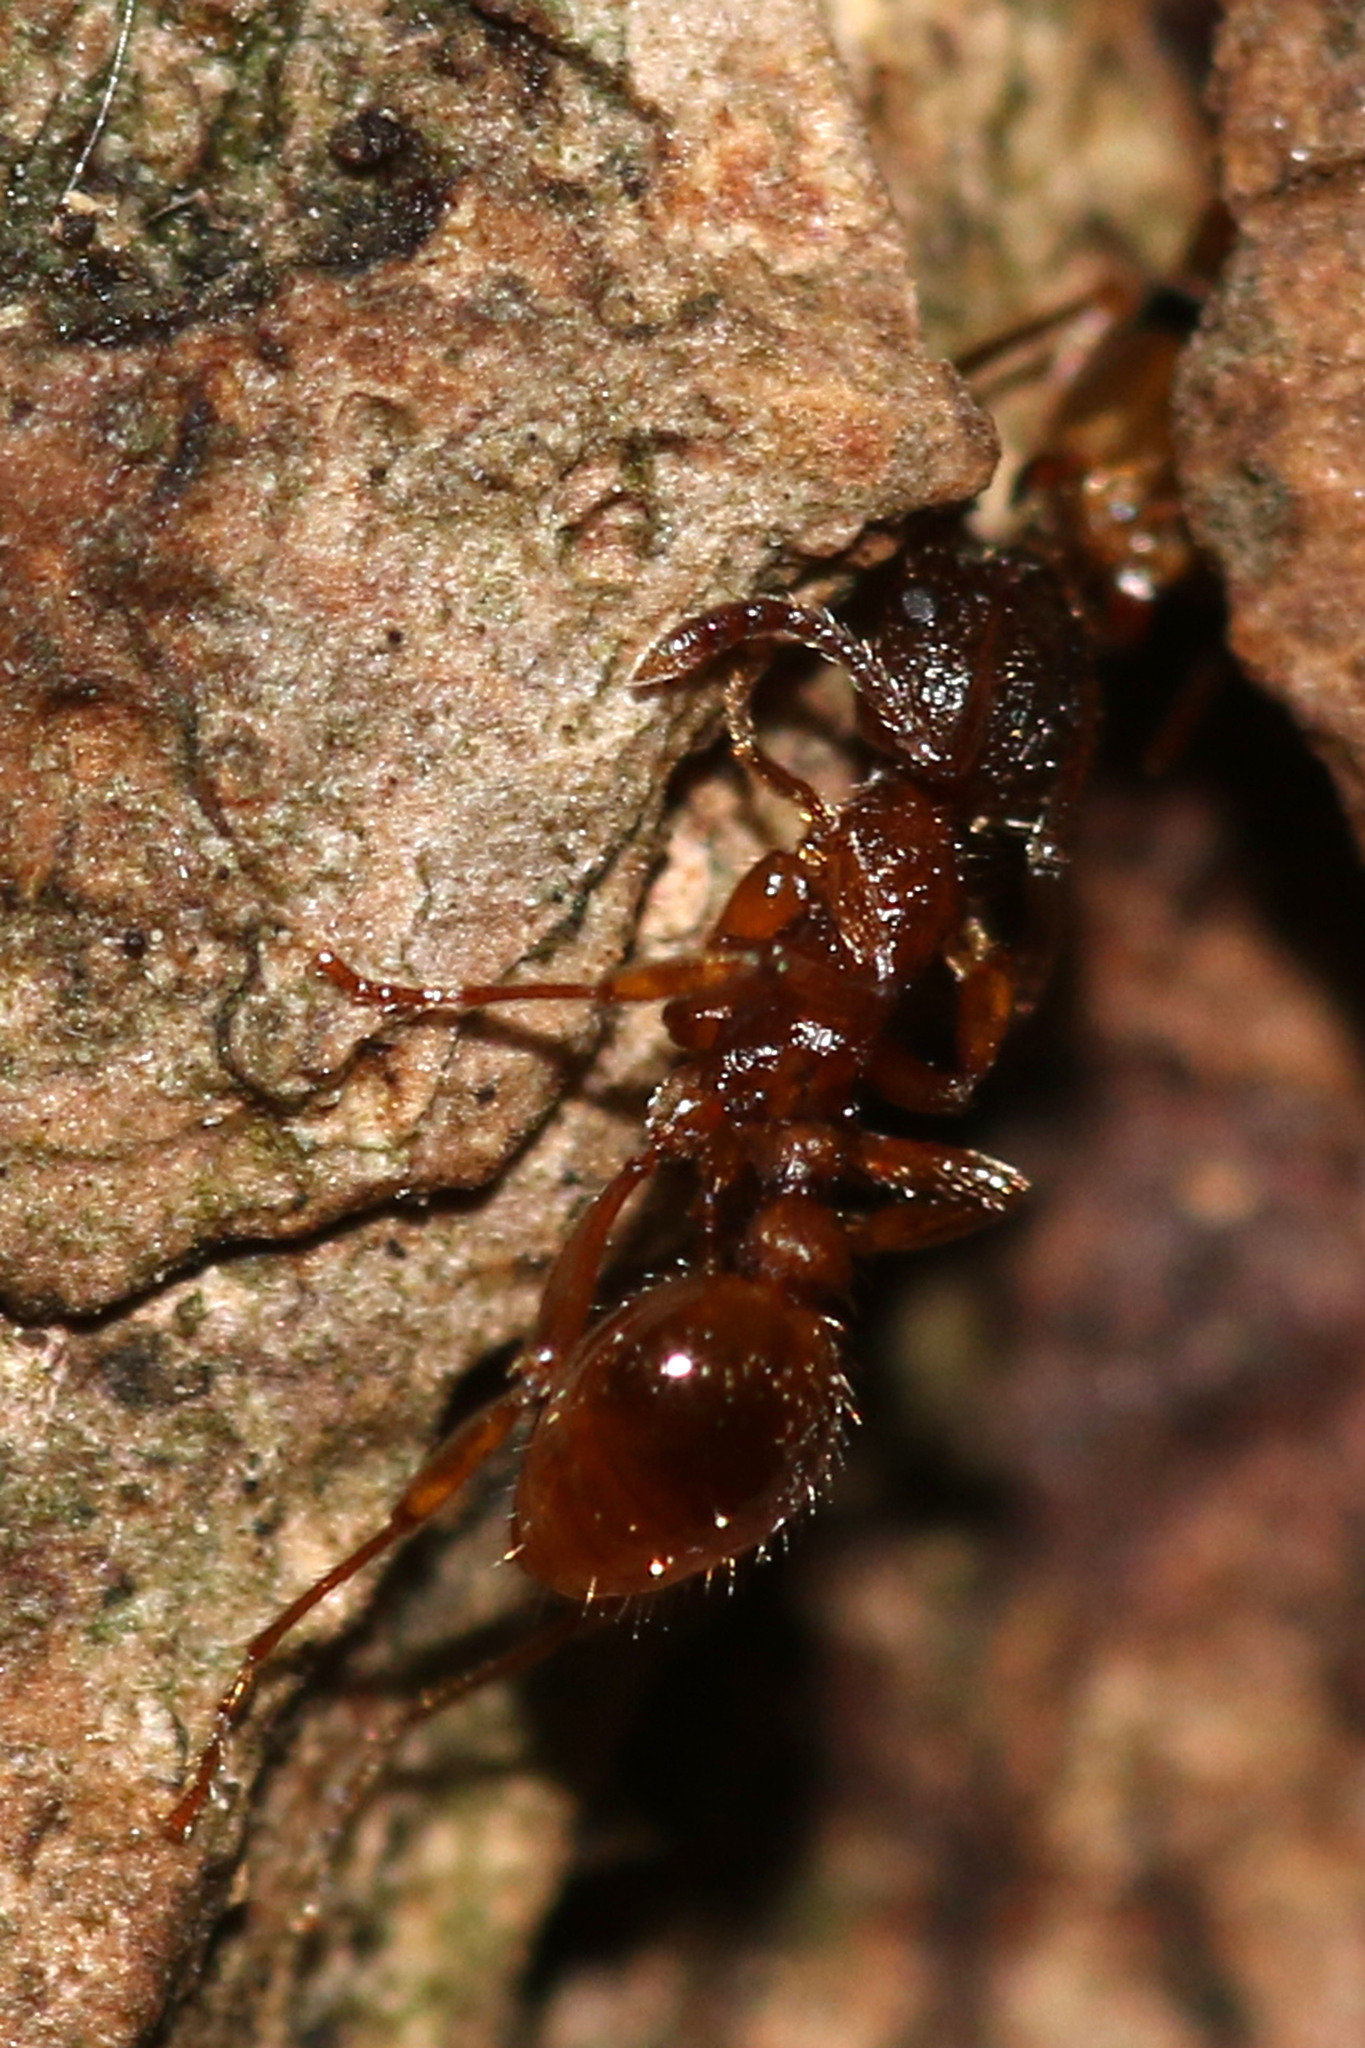}
\end{subfigure}

\vspace{0.1cm}

\begin{subfigure}{0.2\textwidth}
    \includegraphics[width=\textwidth,height=3cm,keepaspectratio=false]{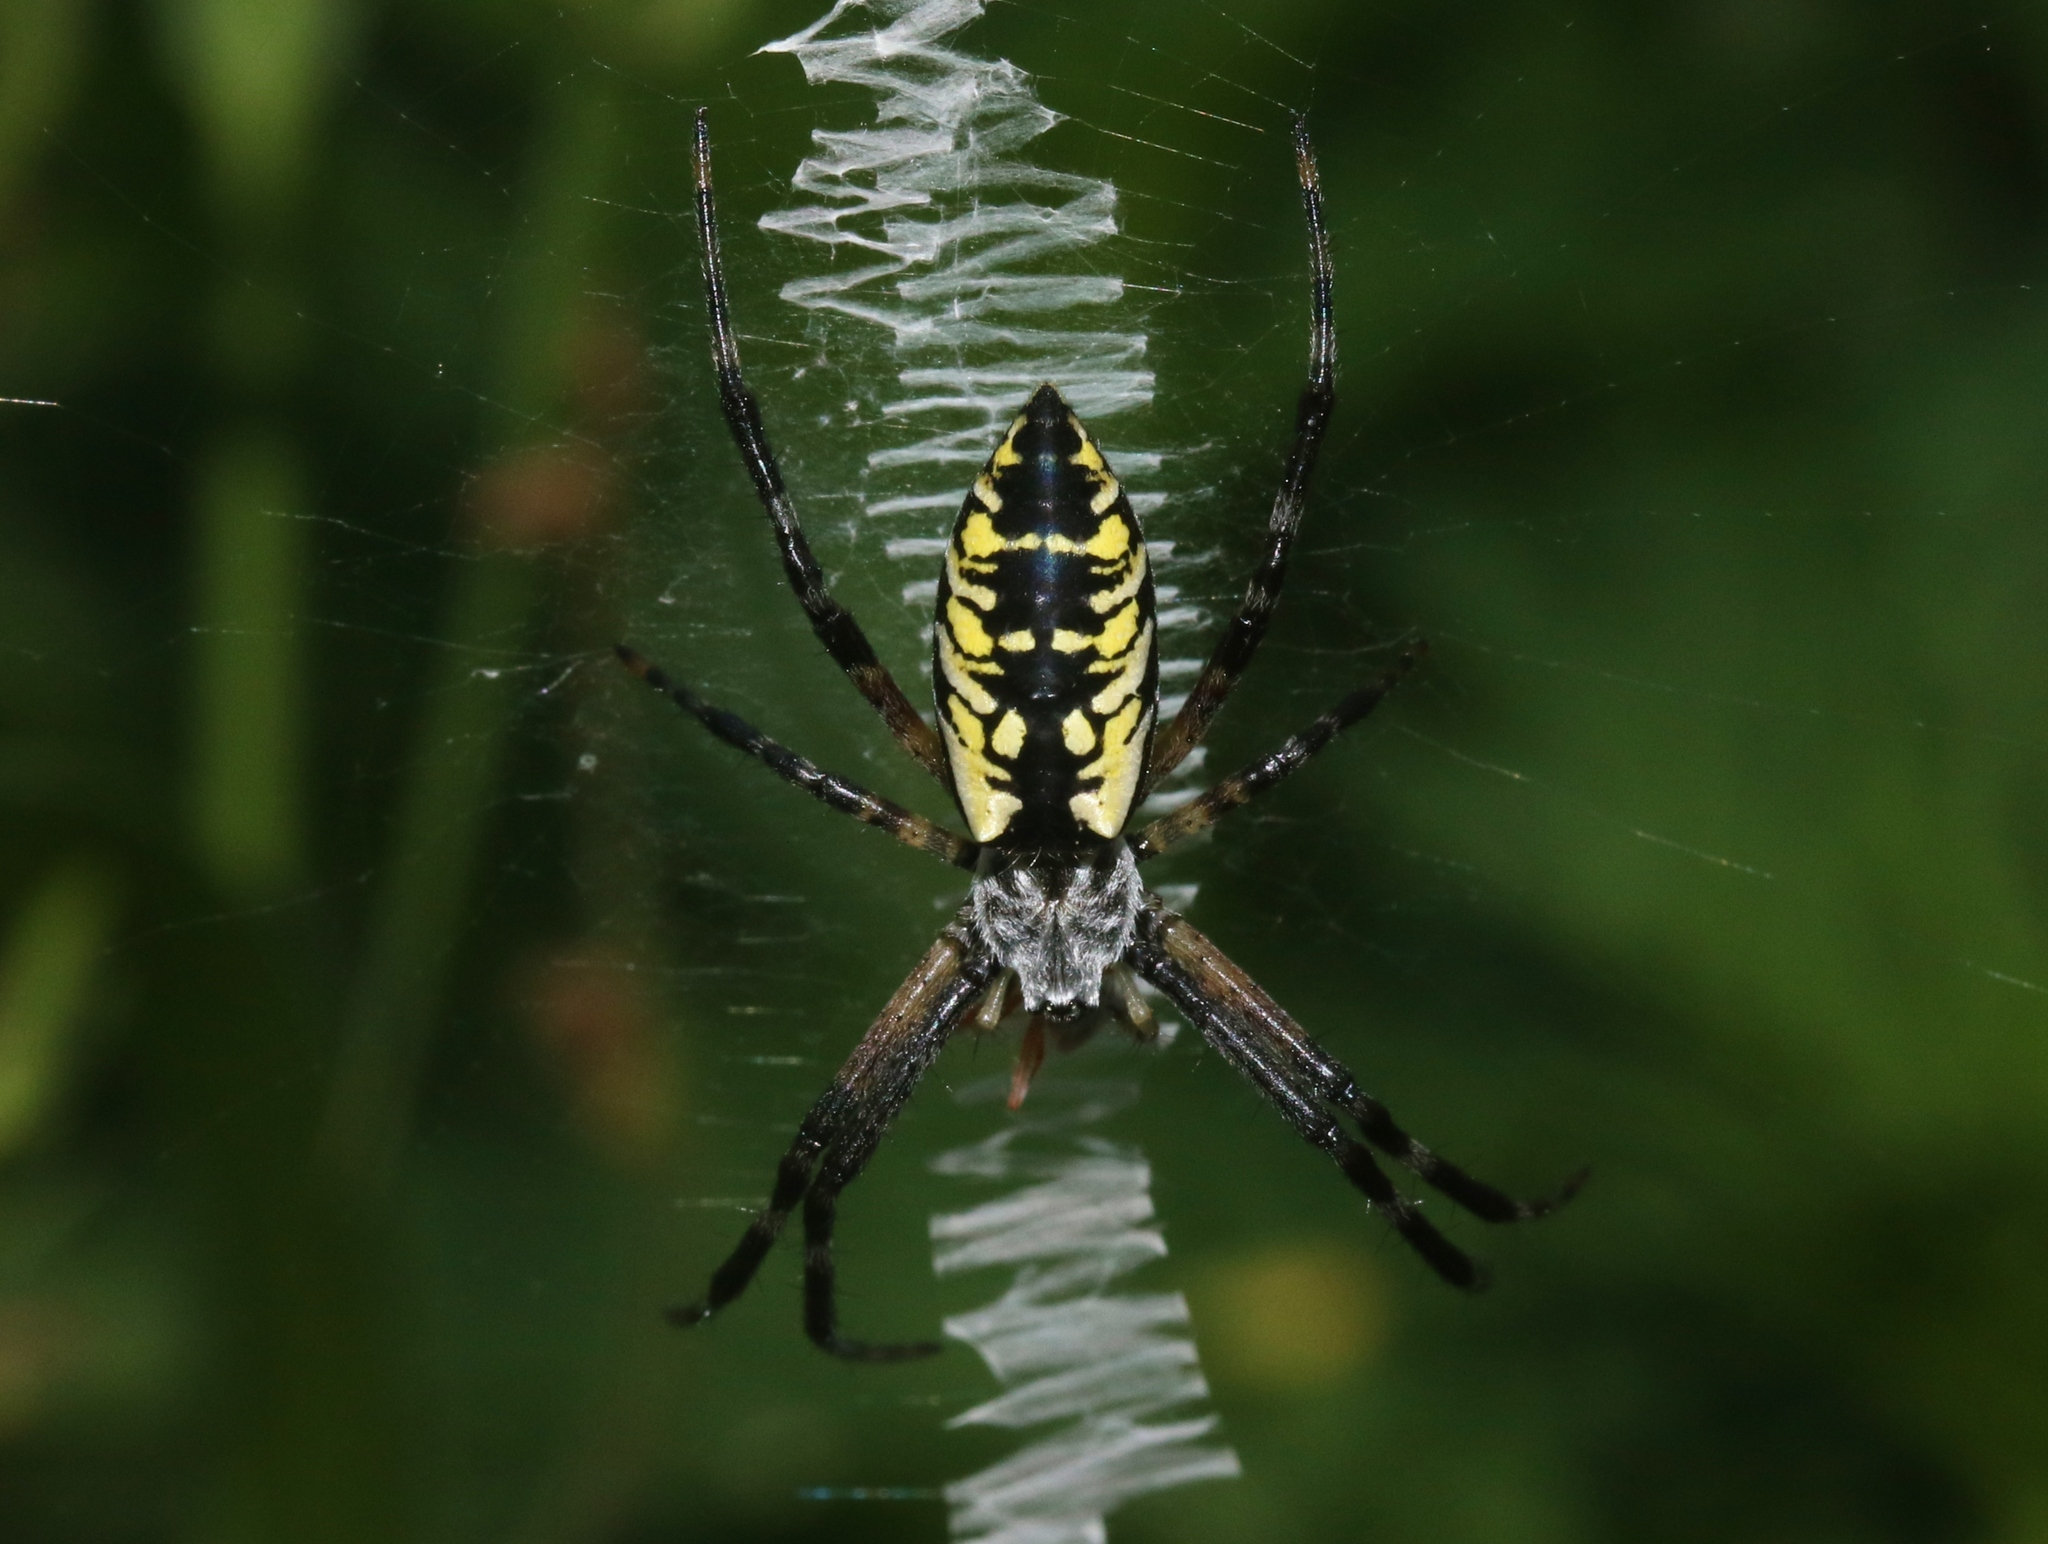}
\end{subfigure}%
\hspace{0.1cm}%
\begin{subfigure}{0.2\textwidth}
    \includegraphics[width=\textwidth,height=3cm,keepaspectratio=false]{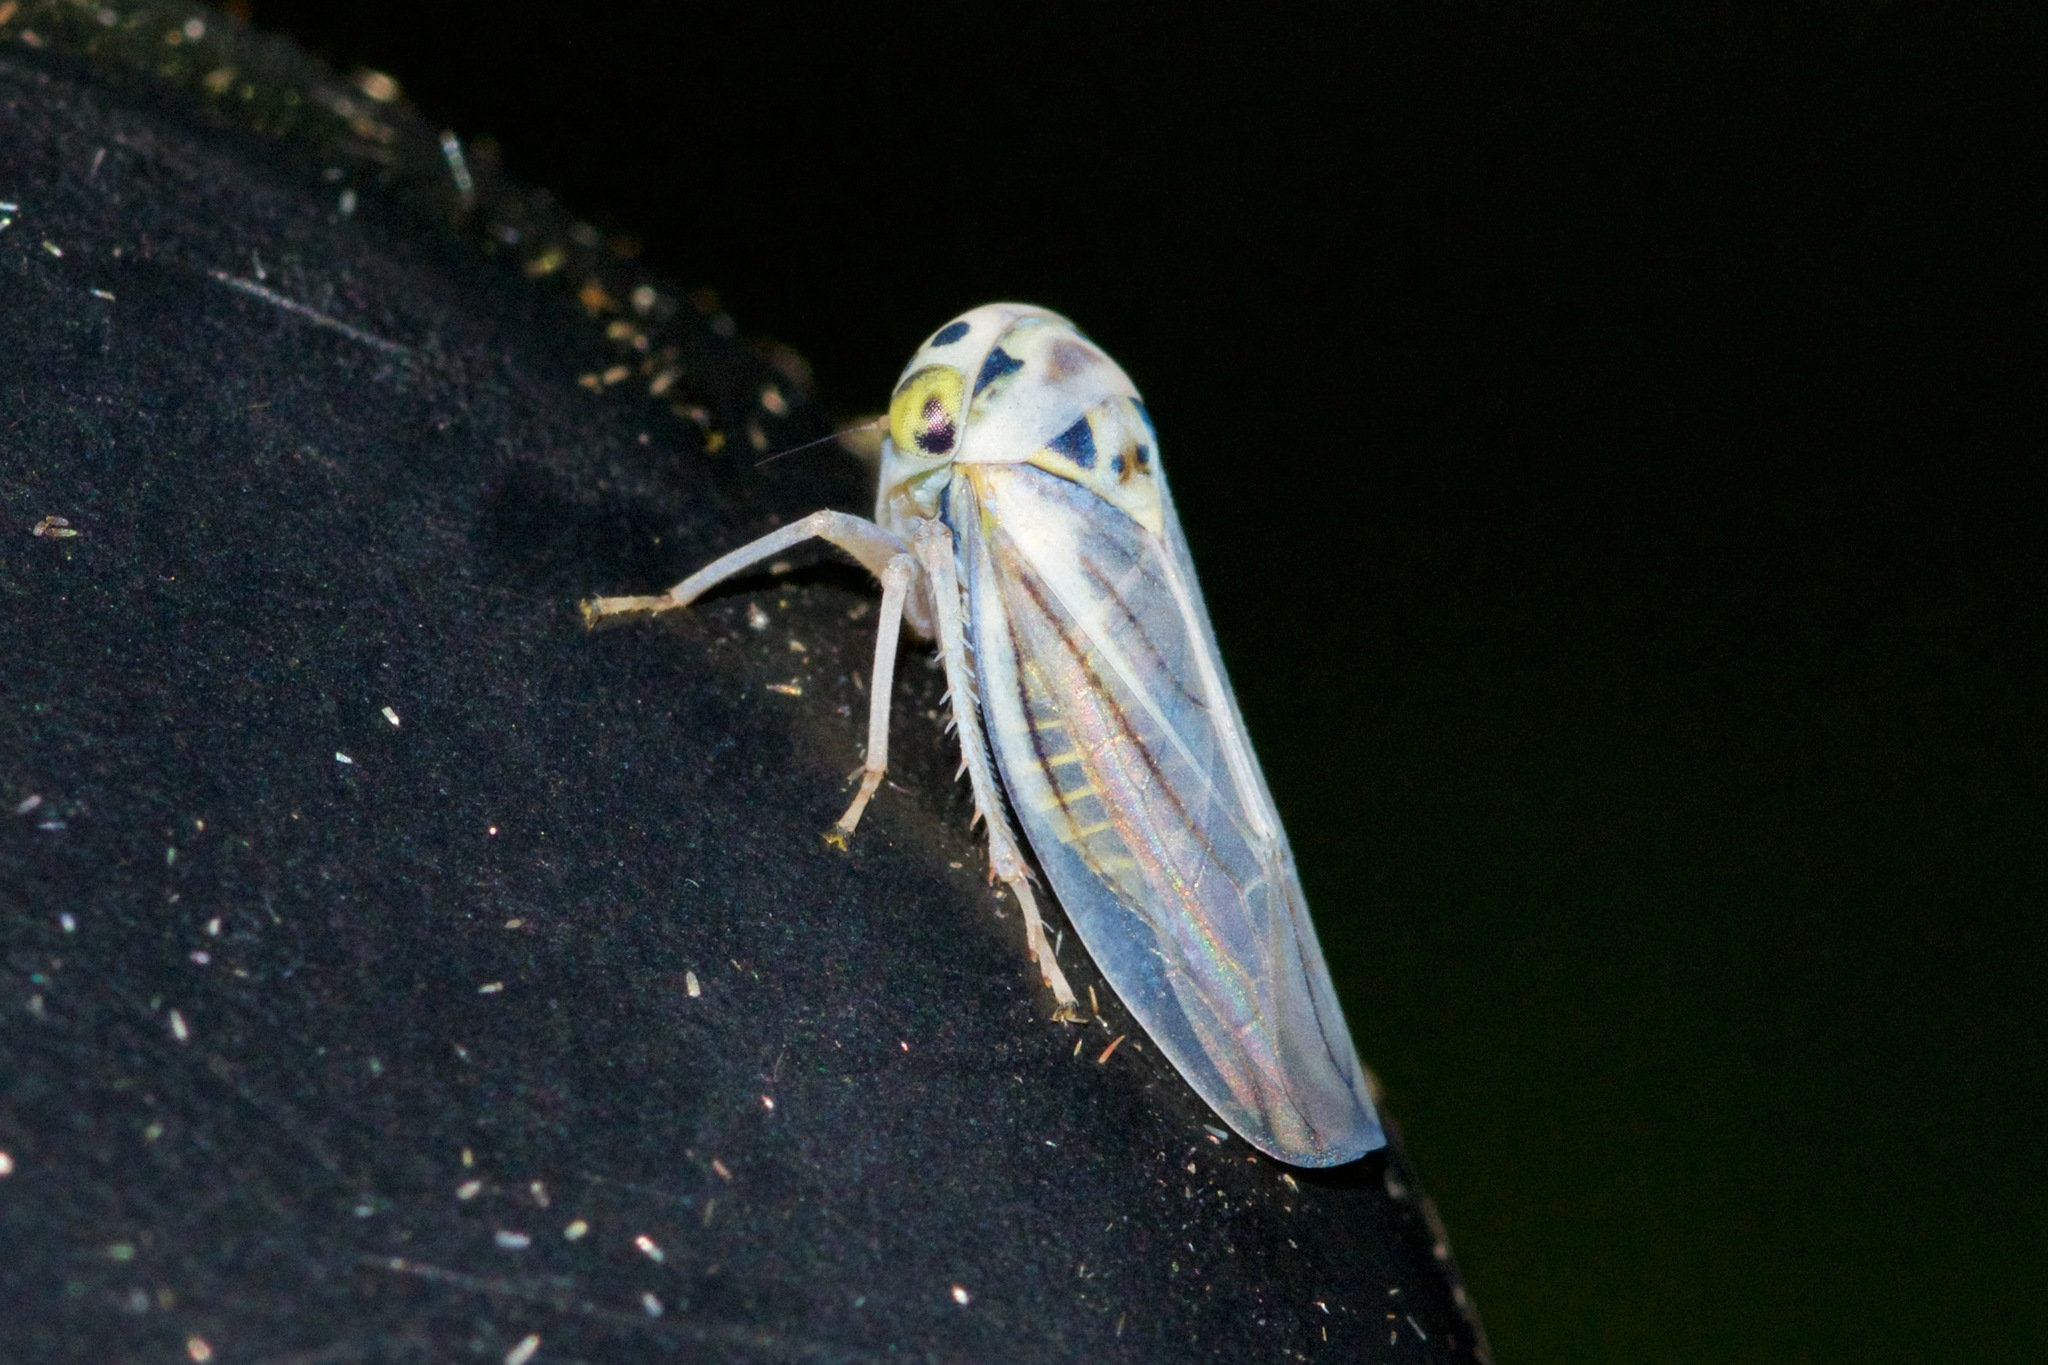}
\end{subfigure}
\caption{Sample images from ArTaxOr dataset showing diverse arthropod species including insects, spiders, and crustaceans with varying scales and natural backgrounds.}
\label{fig:artaxor_samples}
\end{figure}

\begin{figure}[htp]
\centering
\begin{subfigure}{0.2\textwidth}
    \includegraphics[width=\textwidth,height=3cm,keepaspectratio=false]{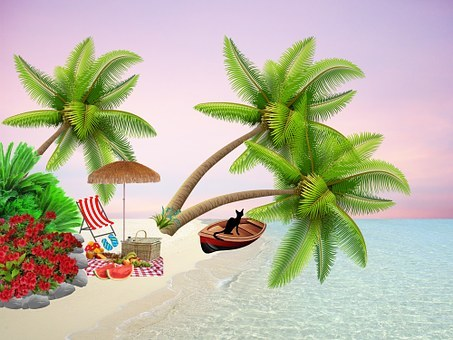}
\end{subfigure}%
\hspace{0.1cm}%
\begin{subfigure}{0.2\textwidth}
    \includegraphics[width=\textwidth,height=3cm,keepaspectratio=false]{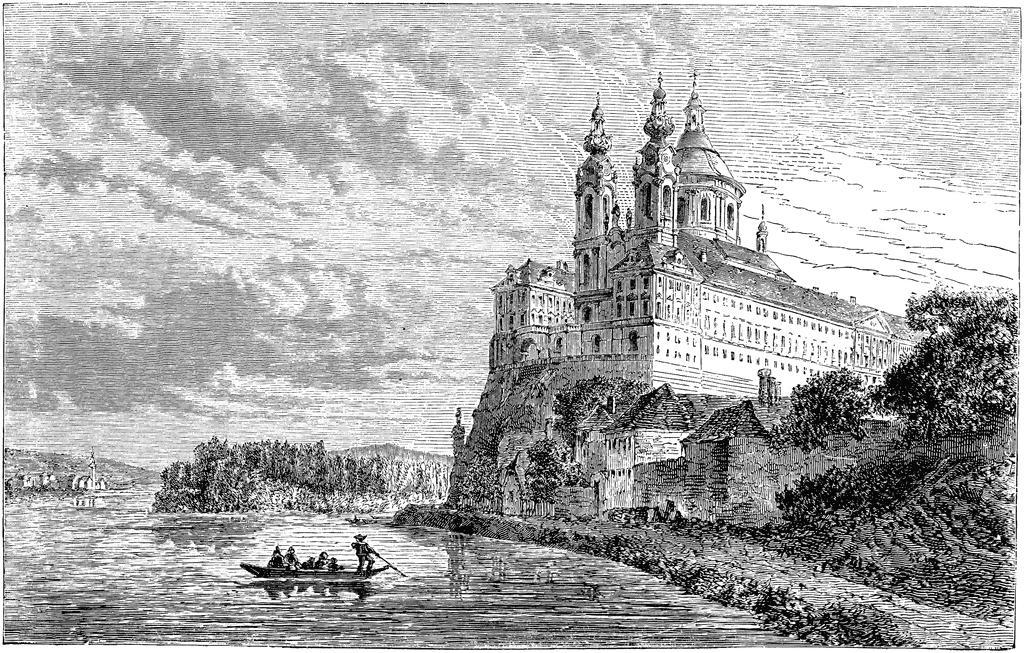}
\end{subfigure}

\vspace{0.1cm}

\begin{subfigure}{0.2\textwidth}
    \includegraphics[width=\textwidth,height=3cm,keepaspectratio=false]{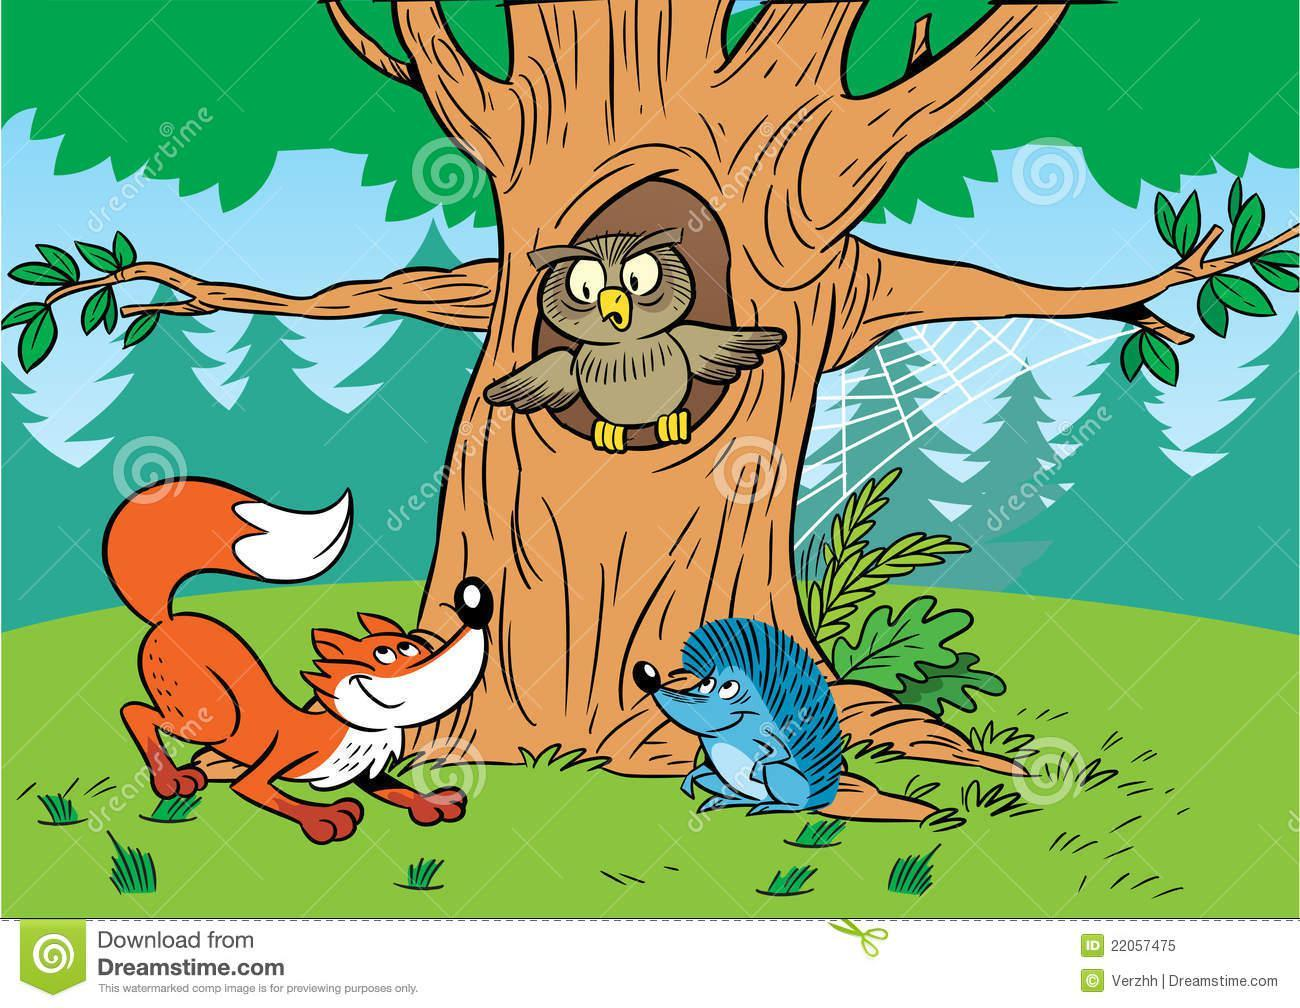}
\end{subfigure}%
\hspace{0.1cm}%
\begin{subfigure}{0.2\textwidth}
    \includegraphics[width=\textwidth,height=3cm,keepaspectratio=false]{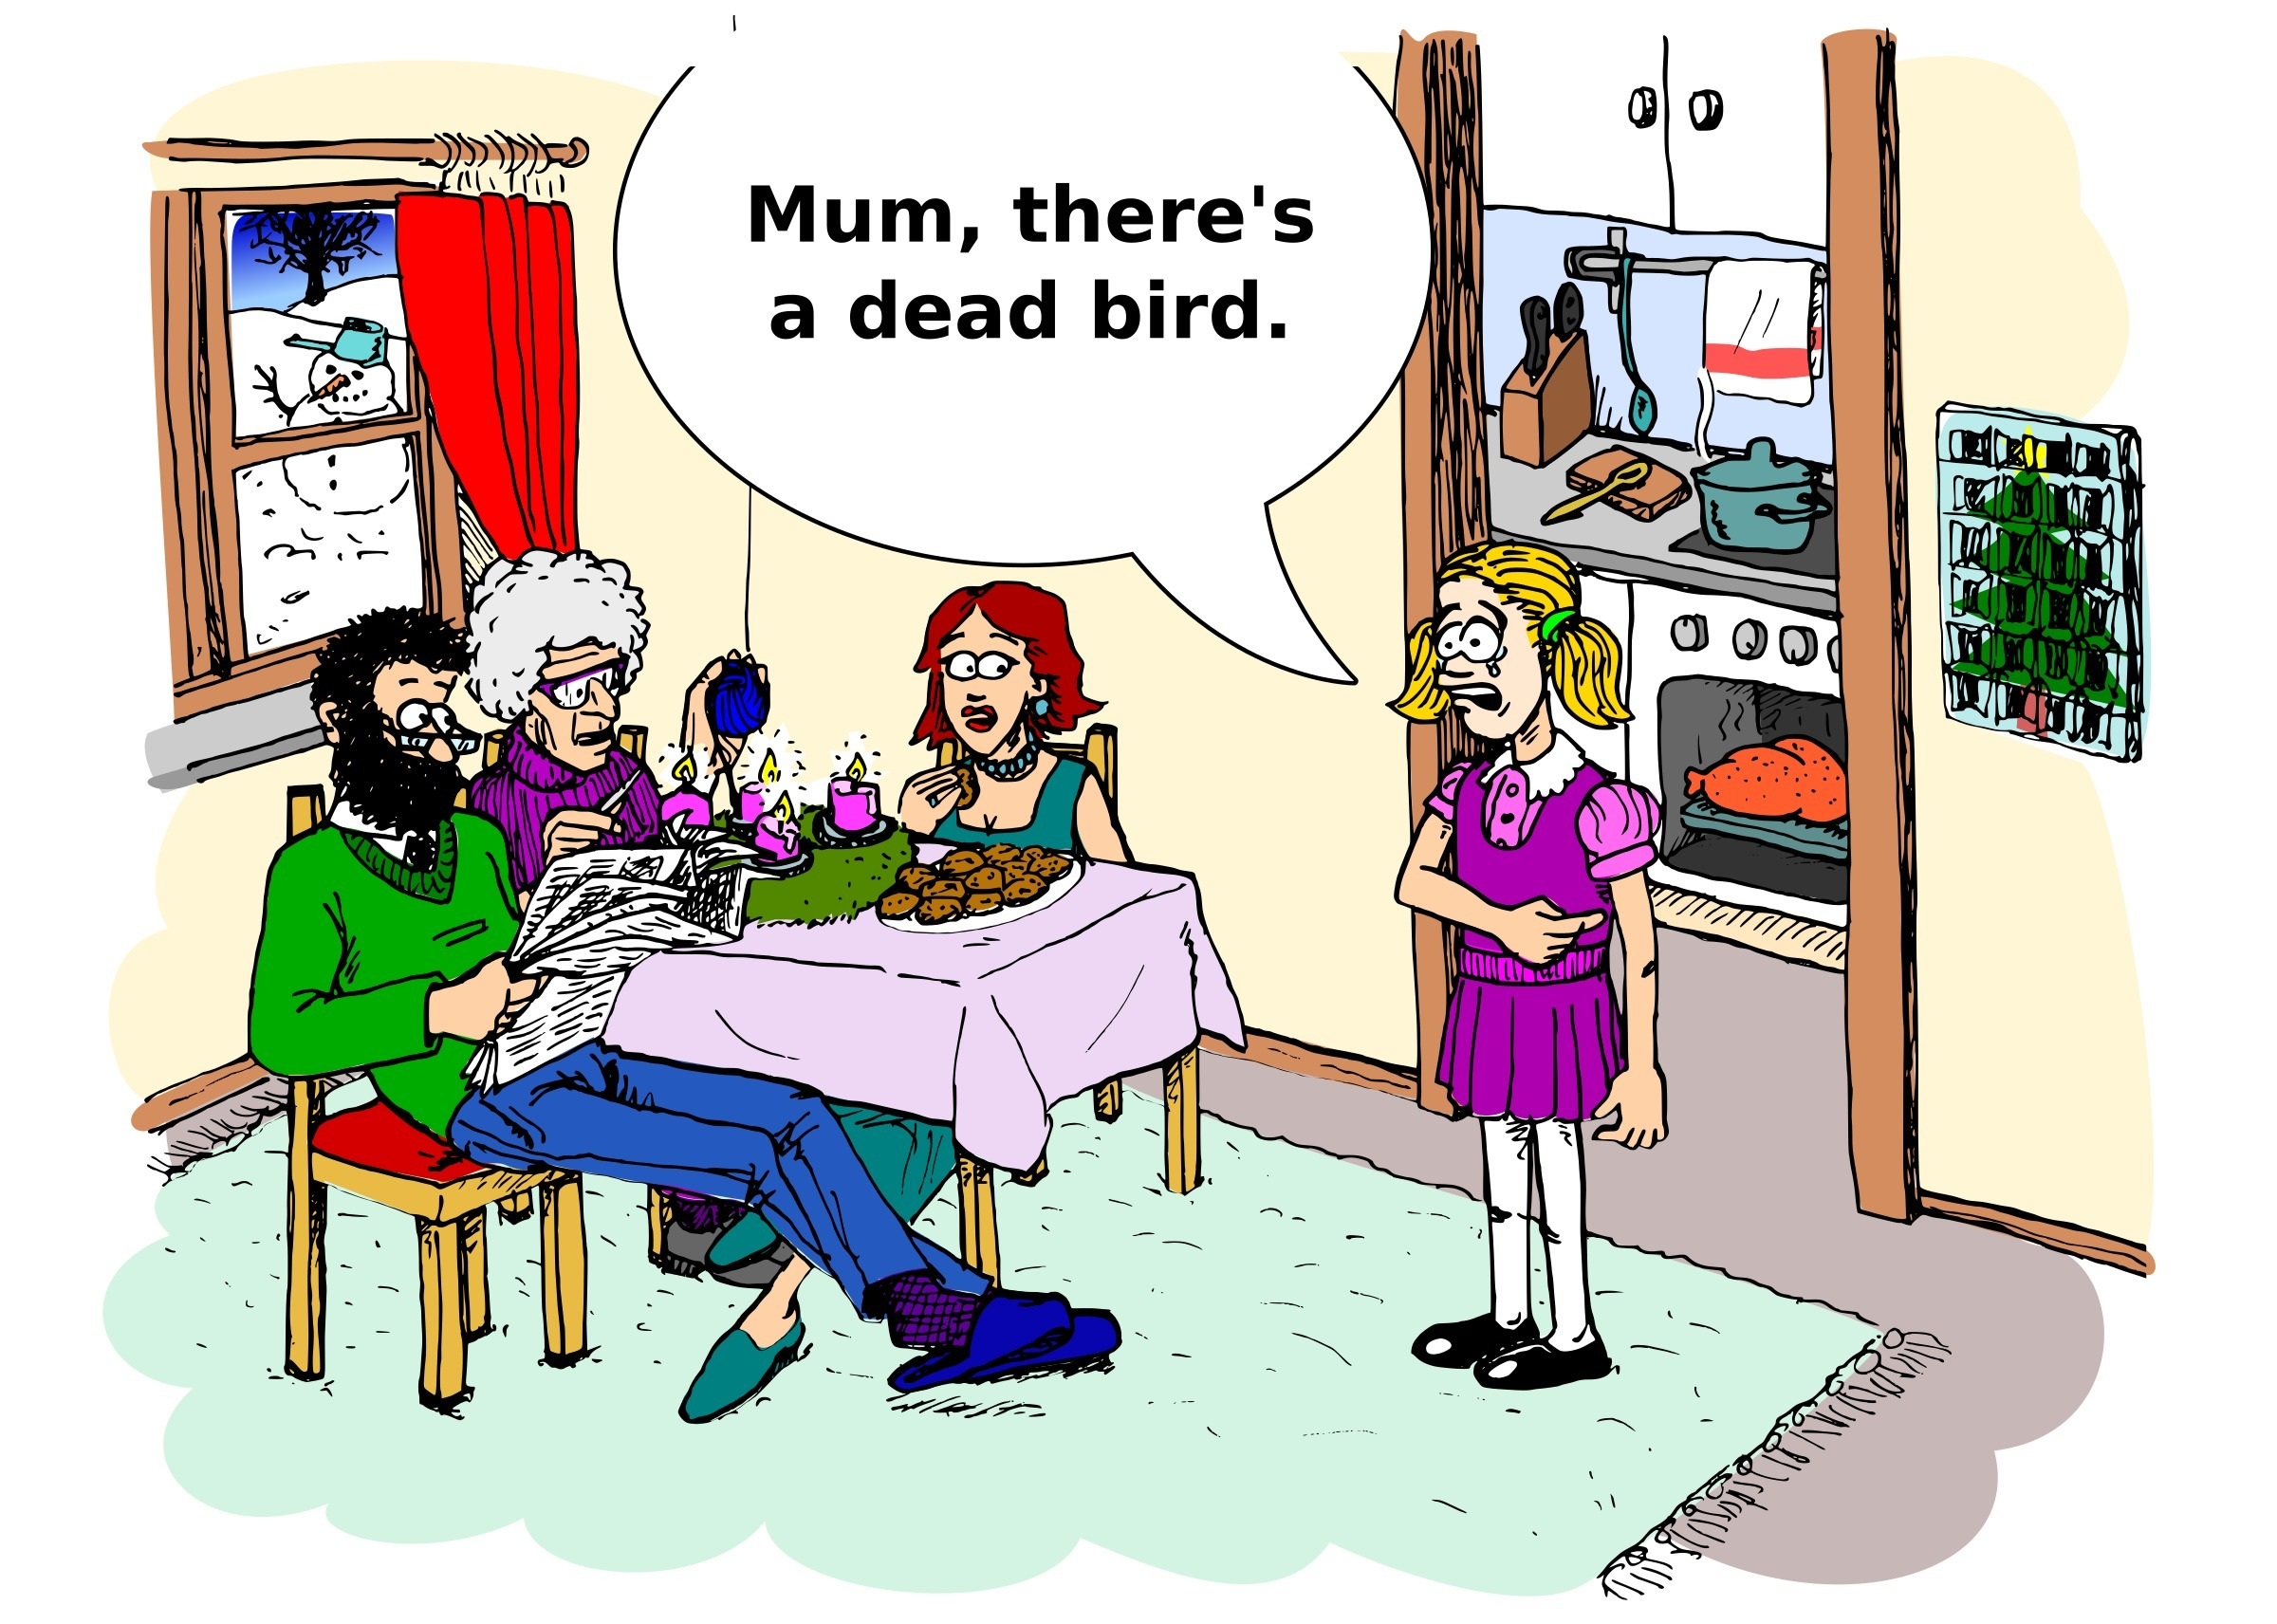}
\end{subfigure}
\caption{Sample images from Clipart1k dataset showing cartoon-style objects with simplified visual features and artistic rendering.}
\label{fig:clipart1k_samples}
\end{figure}

\begin{figure}[h]
\centering
\begin{subfigure}{0.2\textwidth}
    \includegraphics[width=\textwidth,height=3cm,keepaspectratio=false]{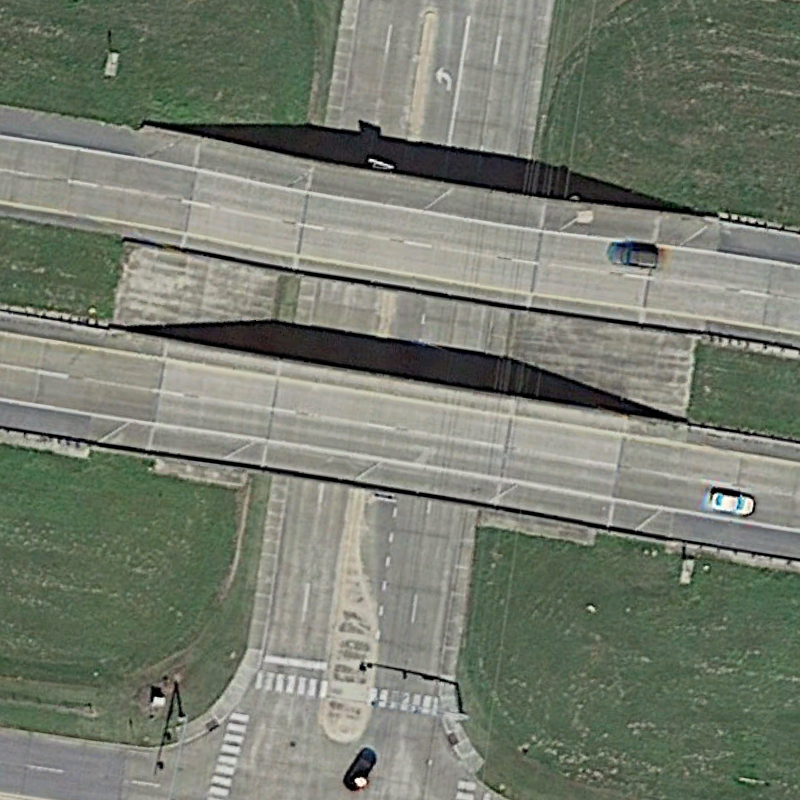}
\end{subfigure}%
\hspace{0.1cm}%
\begin{subfigure}{0.2\textwidth}
    \includegraphics[width=\textwidth,height=3cm,keepaspectratio=false]{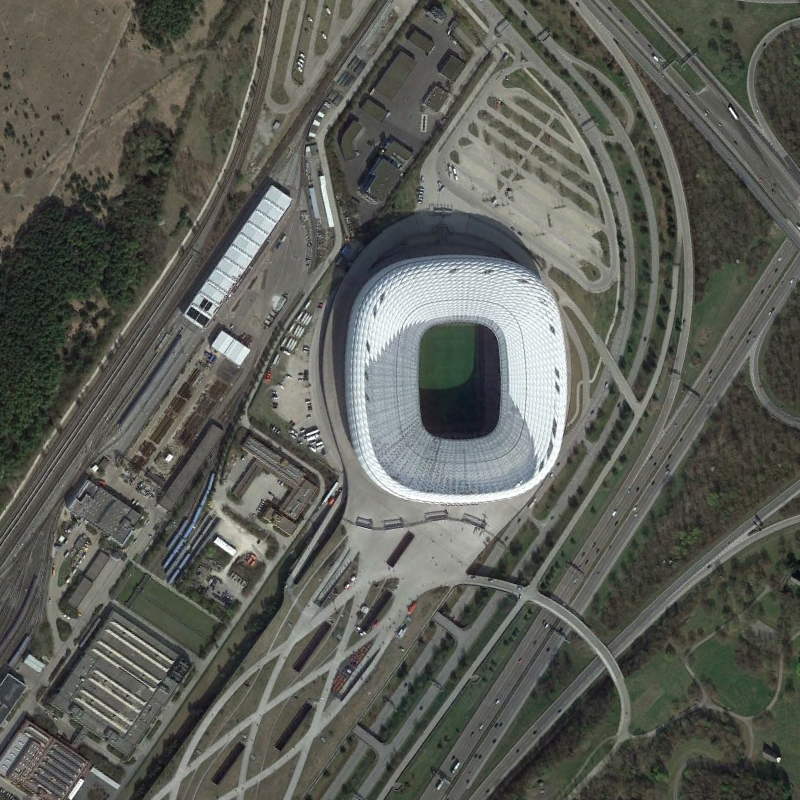}
\end{subfigure}

\vspace{0.1cm}

\begin{subfigure}{0.2\textwidth}
    \includegraphics[width=\textwidth,height=3cm,keepaspectratio=false]{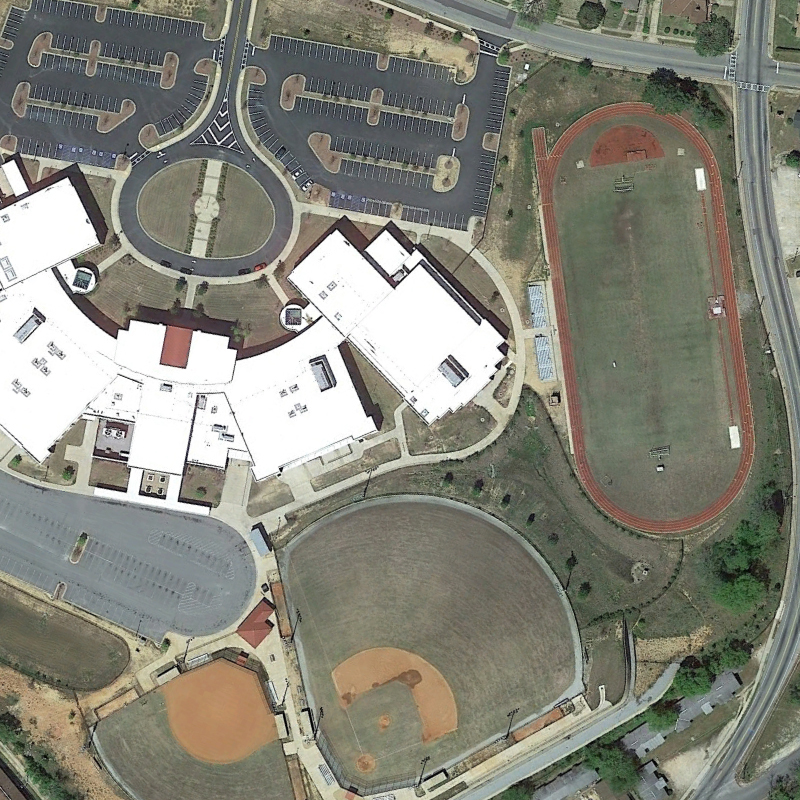}
\end{subfigure}%
\hspace{0.1cm}%
\begin{subfigure}{0.2\textwidth}
    \includegraphics[width=\textwidth,height=3cm,keepaspectratio=false]{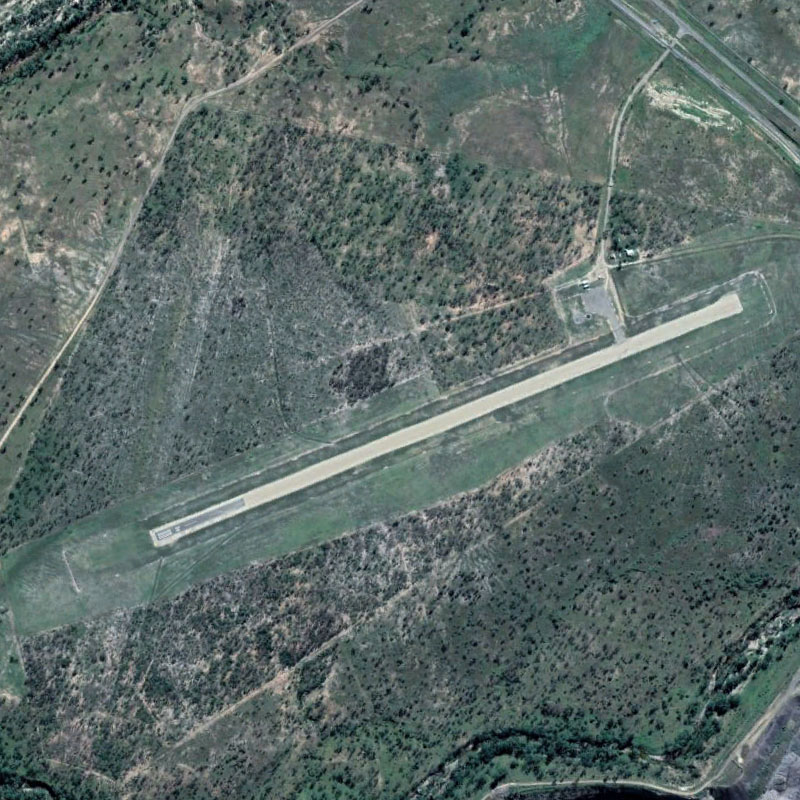}
\end{subfigure}
\caption{Sample images from DIOR dataset featuring remote sensing objects such as airplanes, ships, and golf fields captured from satellite perspectives.}
\label{fig:dior_samples}
\end{figure}

\begin{figure}[h]
\centering
\begin{subfigure}{0.2\textwidth}
    \includegraphics[width=\textwidth,height=3cm,keepaspectratio=false]{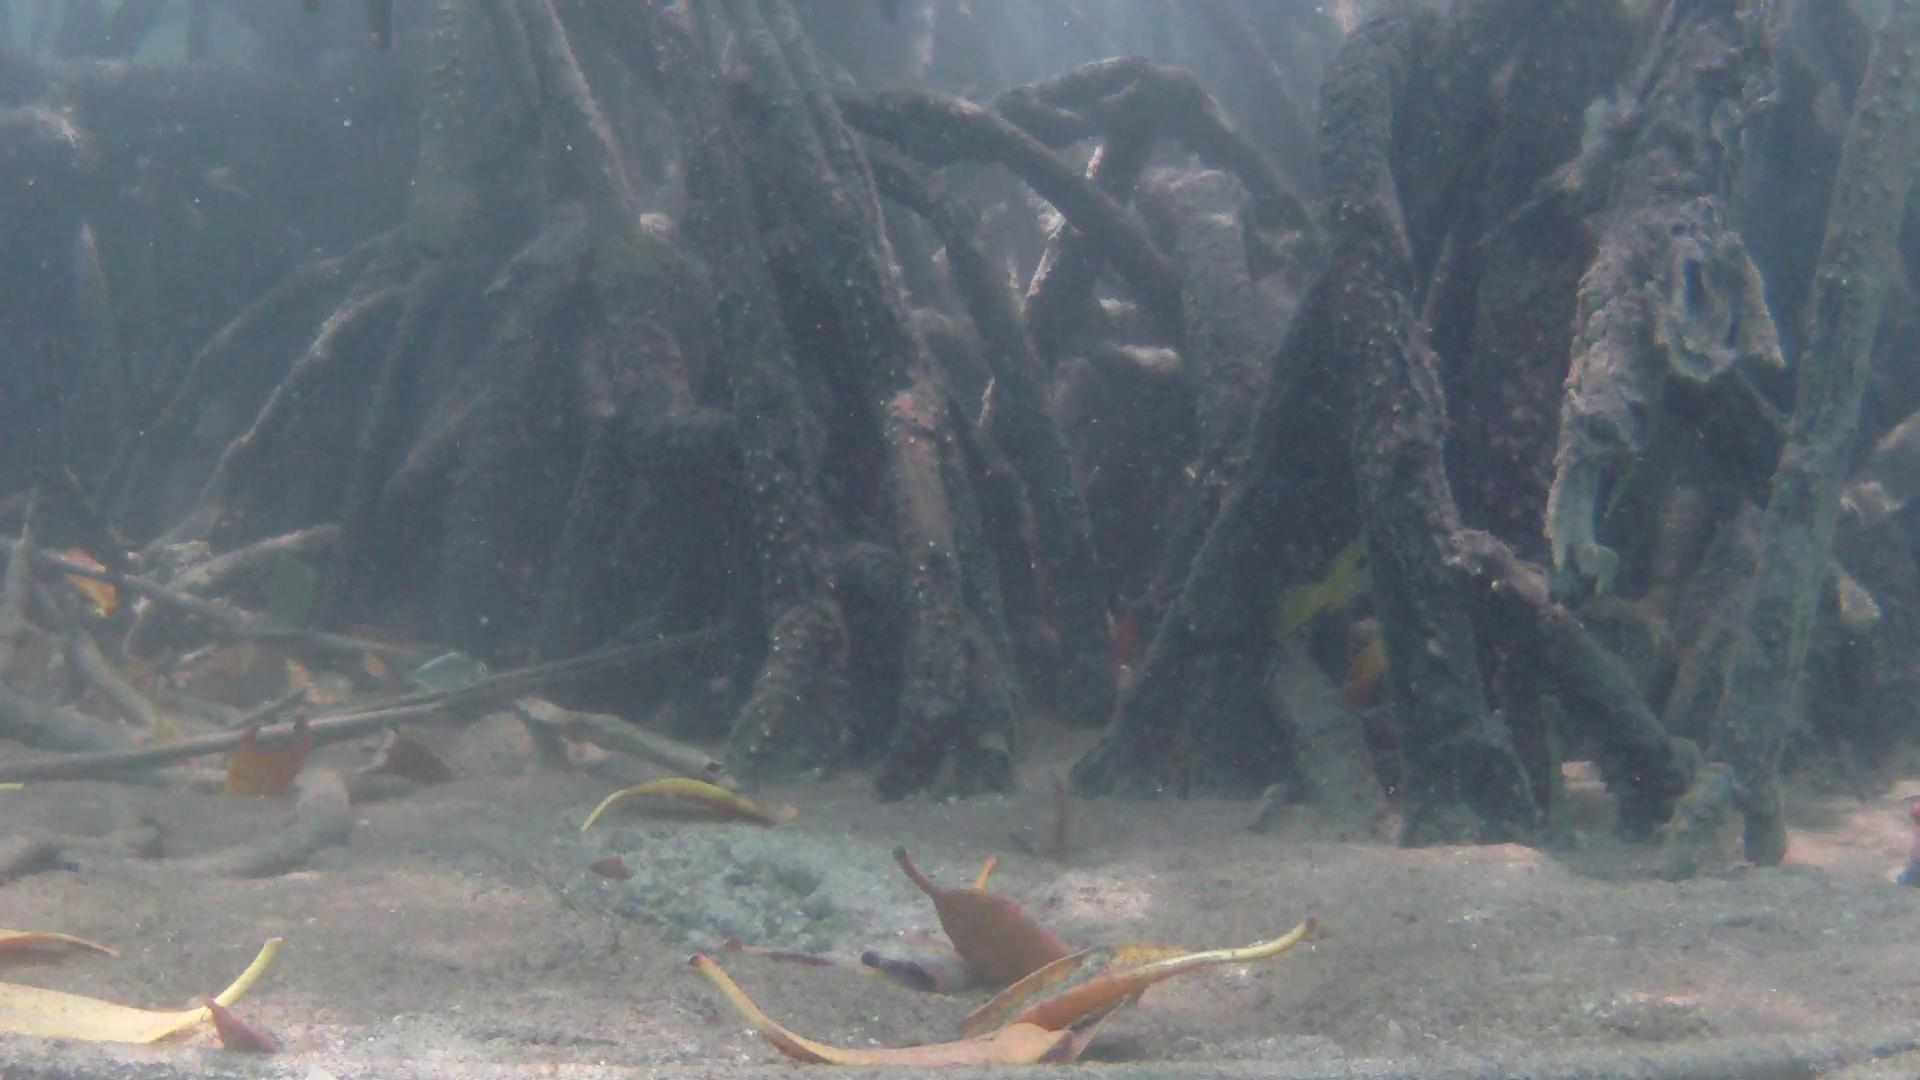}
\end{subfigure}%
\hspace{0.1cm}%
\begin{subfigure}{0.2\textwidth}
    \includegraphics[width=\textwidth,height=3cm,keepaspectratio=false]{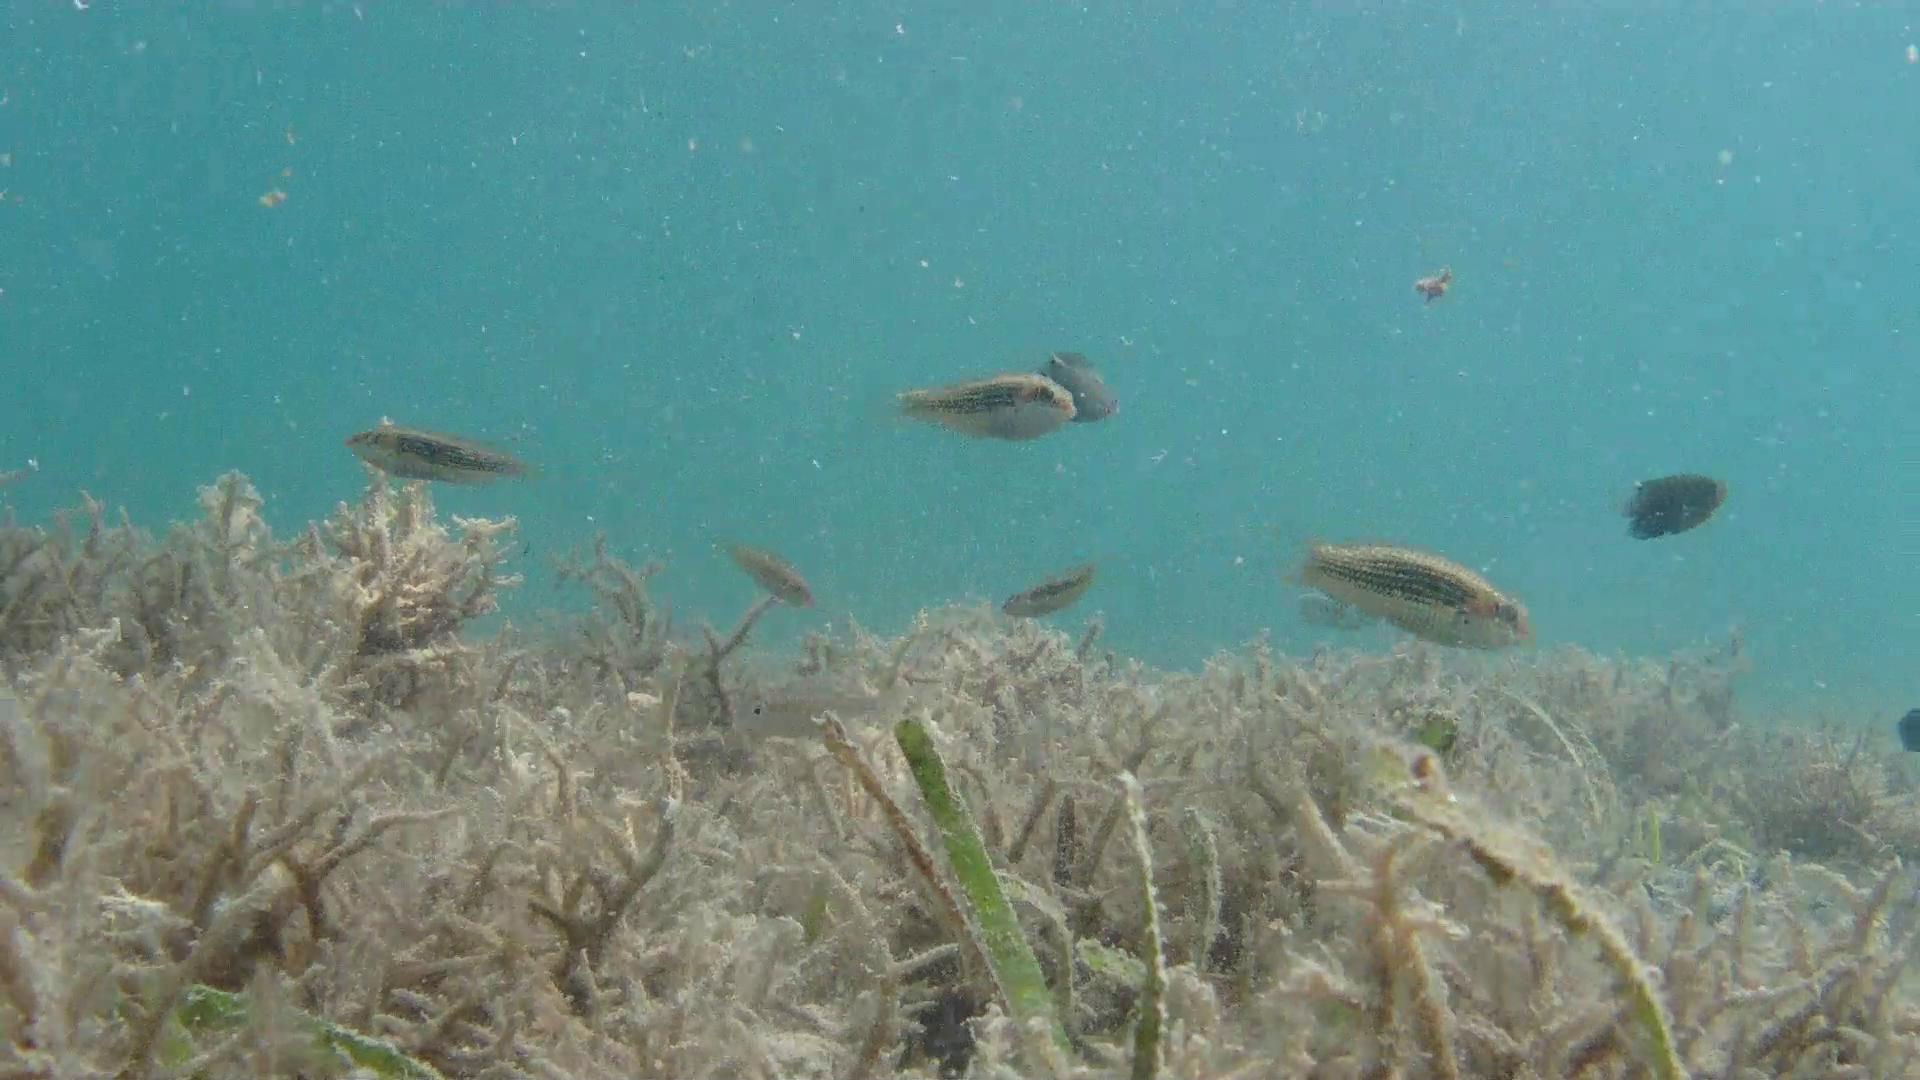}
\end{subfigure}

\vspace{0.1cm}

\begin{subfigure}{0.2\textwidth}
    \includegraphics[width=\textwidth,height=3cm,keepaspectratio=false]{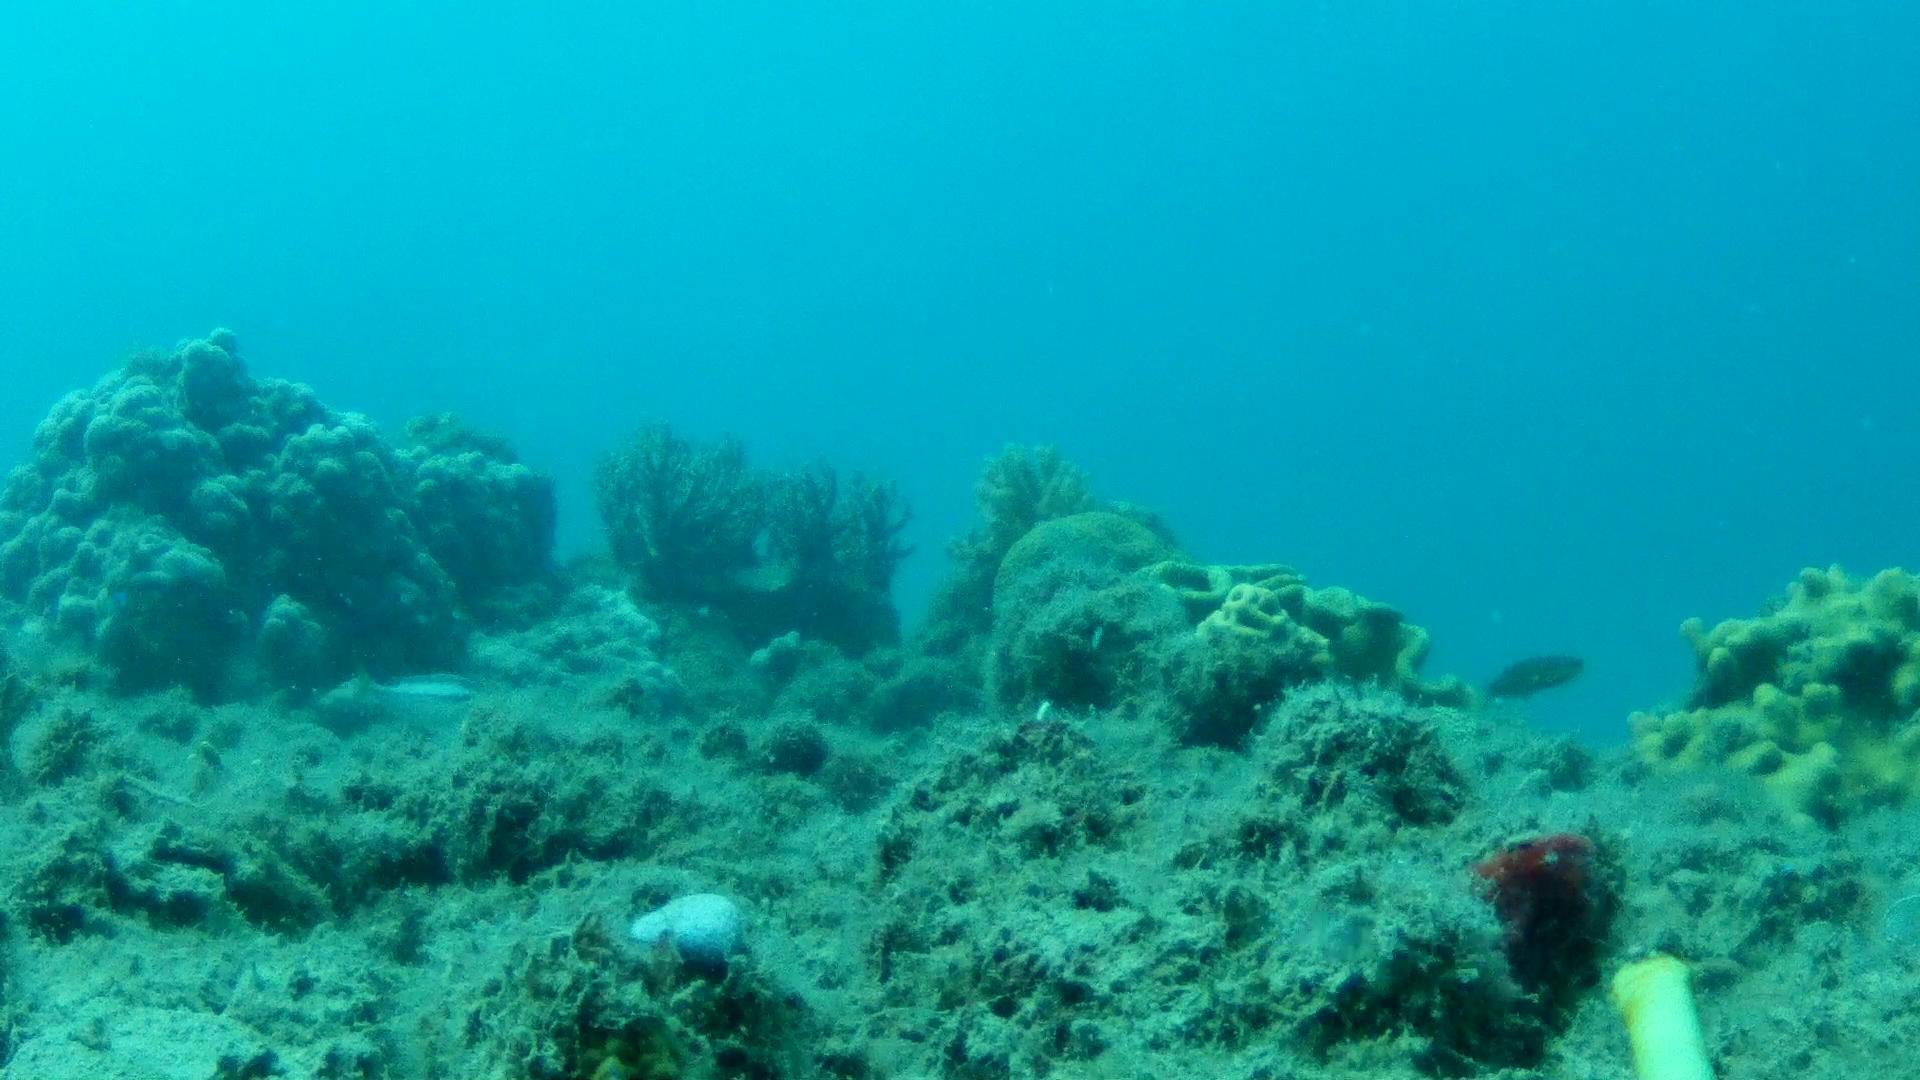}
\end{subfigure}%
\hspace{0.1cm}%
\begin{subfigure}{0.2\textwidth}
    \includegraphics[width=\textwidth,height=3cm,keepaspectratio=false]{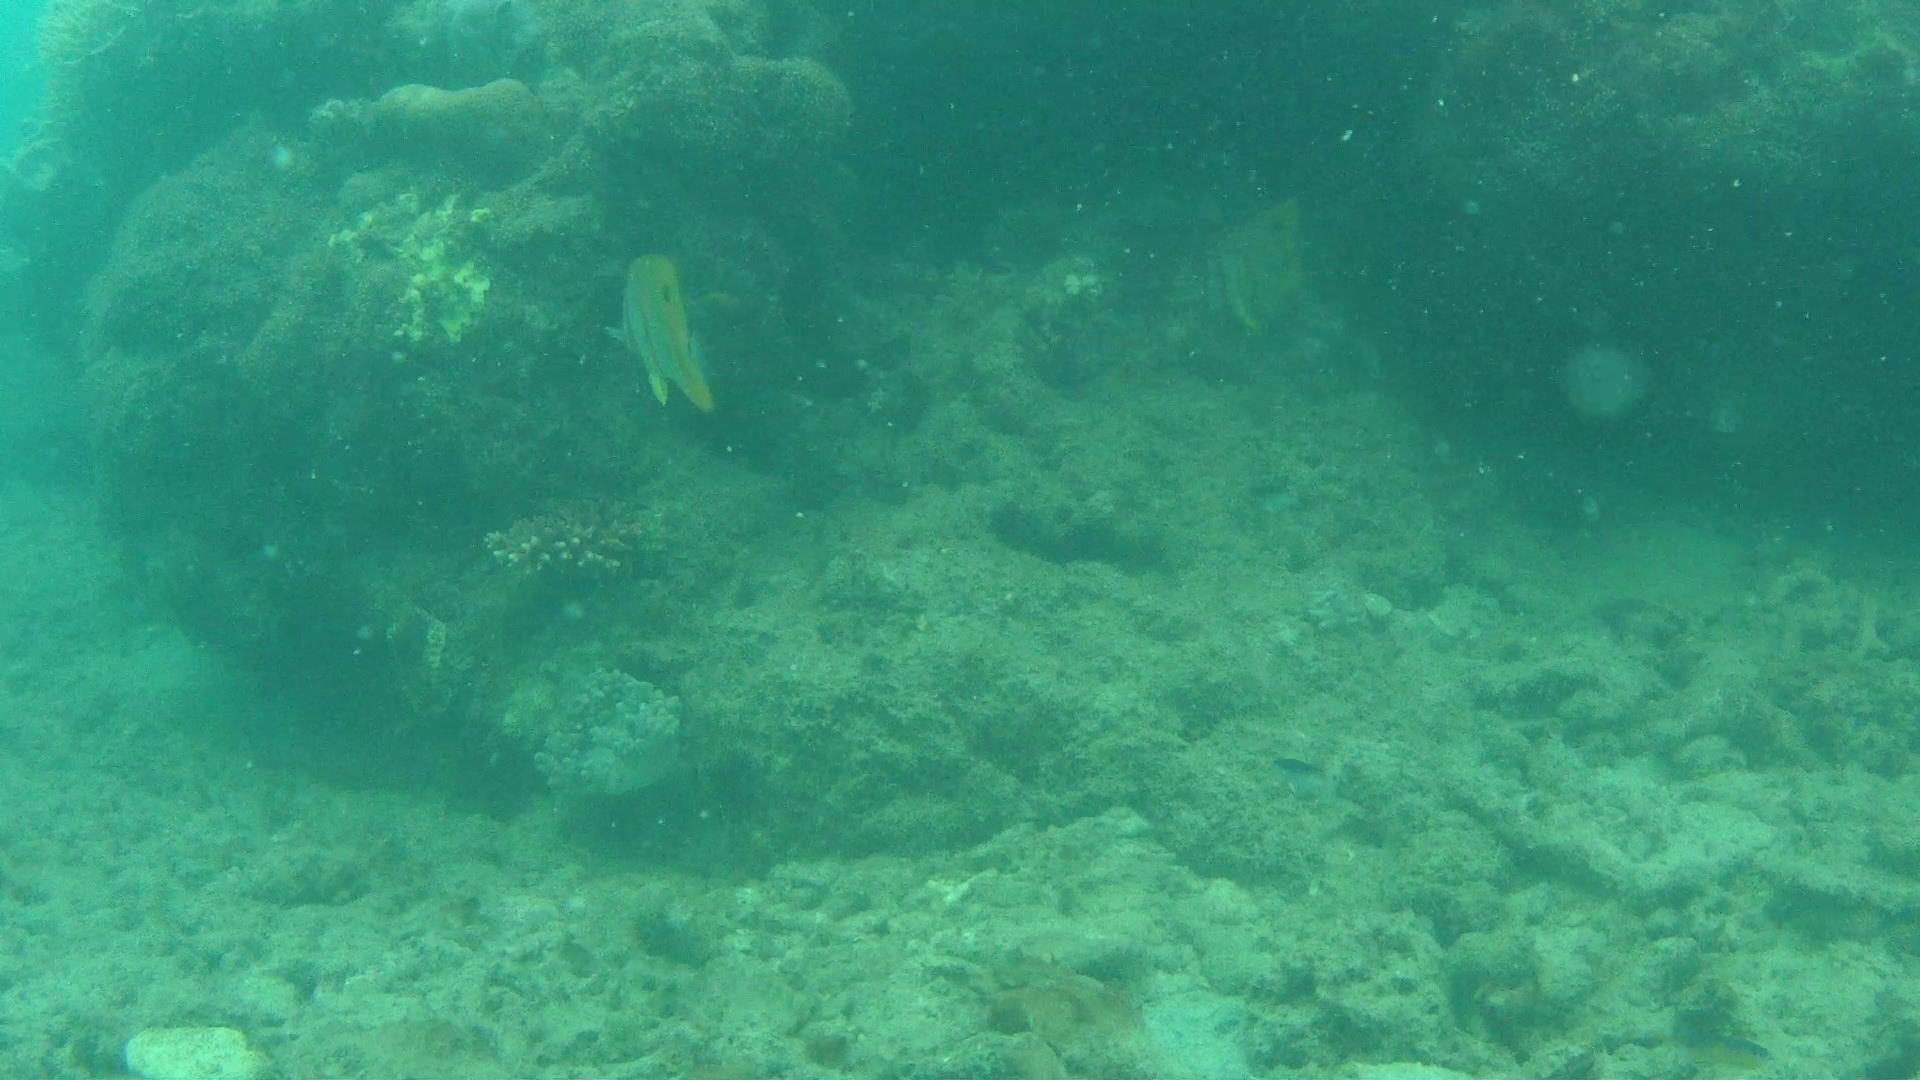}
\end{subfigure}
\caption{Sample images from DeepFish dataset featuring underwater fish detection with challenging lighting conditions and water distortion effects.}
\label{fig:deepfish_samples}
\end{figure}

\begin{figure}[h]
\centering
\begin{subfigure}{0.2\textwidth}
    \includegraphics[width=\textwidth,height=3cm,keepaspectratio=false]{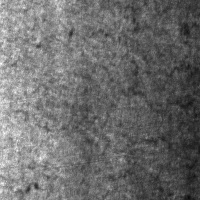}
\end{subfigure}%
\hspace{0.1cm}%
\begin{subfigure}{0.2\textwidth}
    \includegraphics[width=\textwidth,height=3cm,keepaspectratio=false]{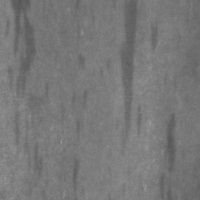}
\end{subfigure}

\vspace{0.1cm}

\begin{subfigure}{0.2\textwidth}
    \includegraphics[width=\textwidth,height=3cm,keepaspectratio=false]{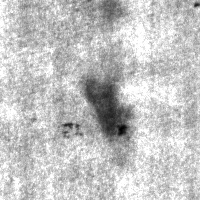}
\end{subfigure}%
\hspace{0.1cm}%
\begin{subfigure}{0.2\textwidth}
    \includegraphics[width=\textwidth,height=3cm,keepaspectratio=false]{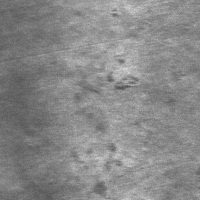}
\end{subfigure}
\caption{Sample images from NEU-DET dataset showing industrial surface defects with subtle visual patterns and varying scales.}
\label{fig:neudet_samples}
\end{figure}

\begin{figure}[h]
\centering
\begin{subfigure}{0.2\textwidth}
    \includegraphics[width=\textwidth,height=3cm,keepaspectratio=false]{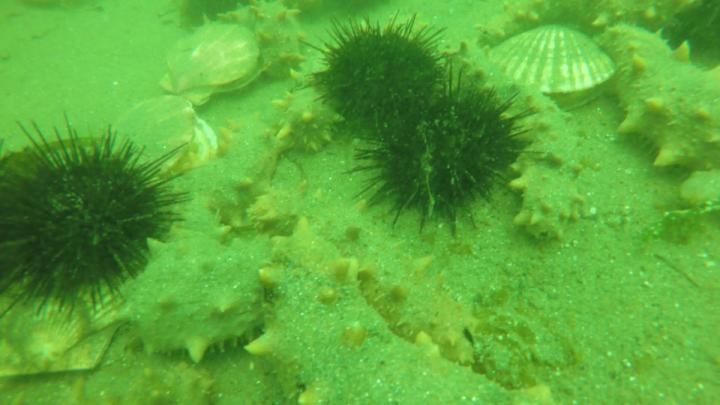}
\end{subfigure}%
\hspace{0.1cm}%
\begin{subfigure}{0.2\textwidth}
    \includegraphics[width=\textwidth,height=3cm,keepaspectratio=false]{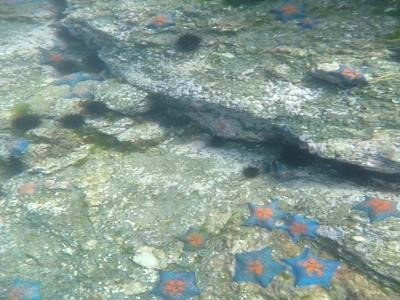}
\end{subfigure}

\vspace{0.1cm}

\begin{subfigure}{0.2\textwidth}
    \includegraphics[width=\textwidth,height=3cm,keepaspectratio=false]{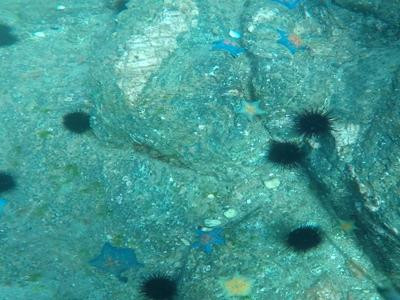}
\end{subfigure}%
\hspace{0.1cm}%
\begin{subfigure}{0.2\textwidth}
    \includegraphics[width=\textwidth,height=3cm,keepaspectratio=false]{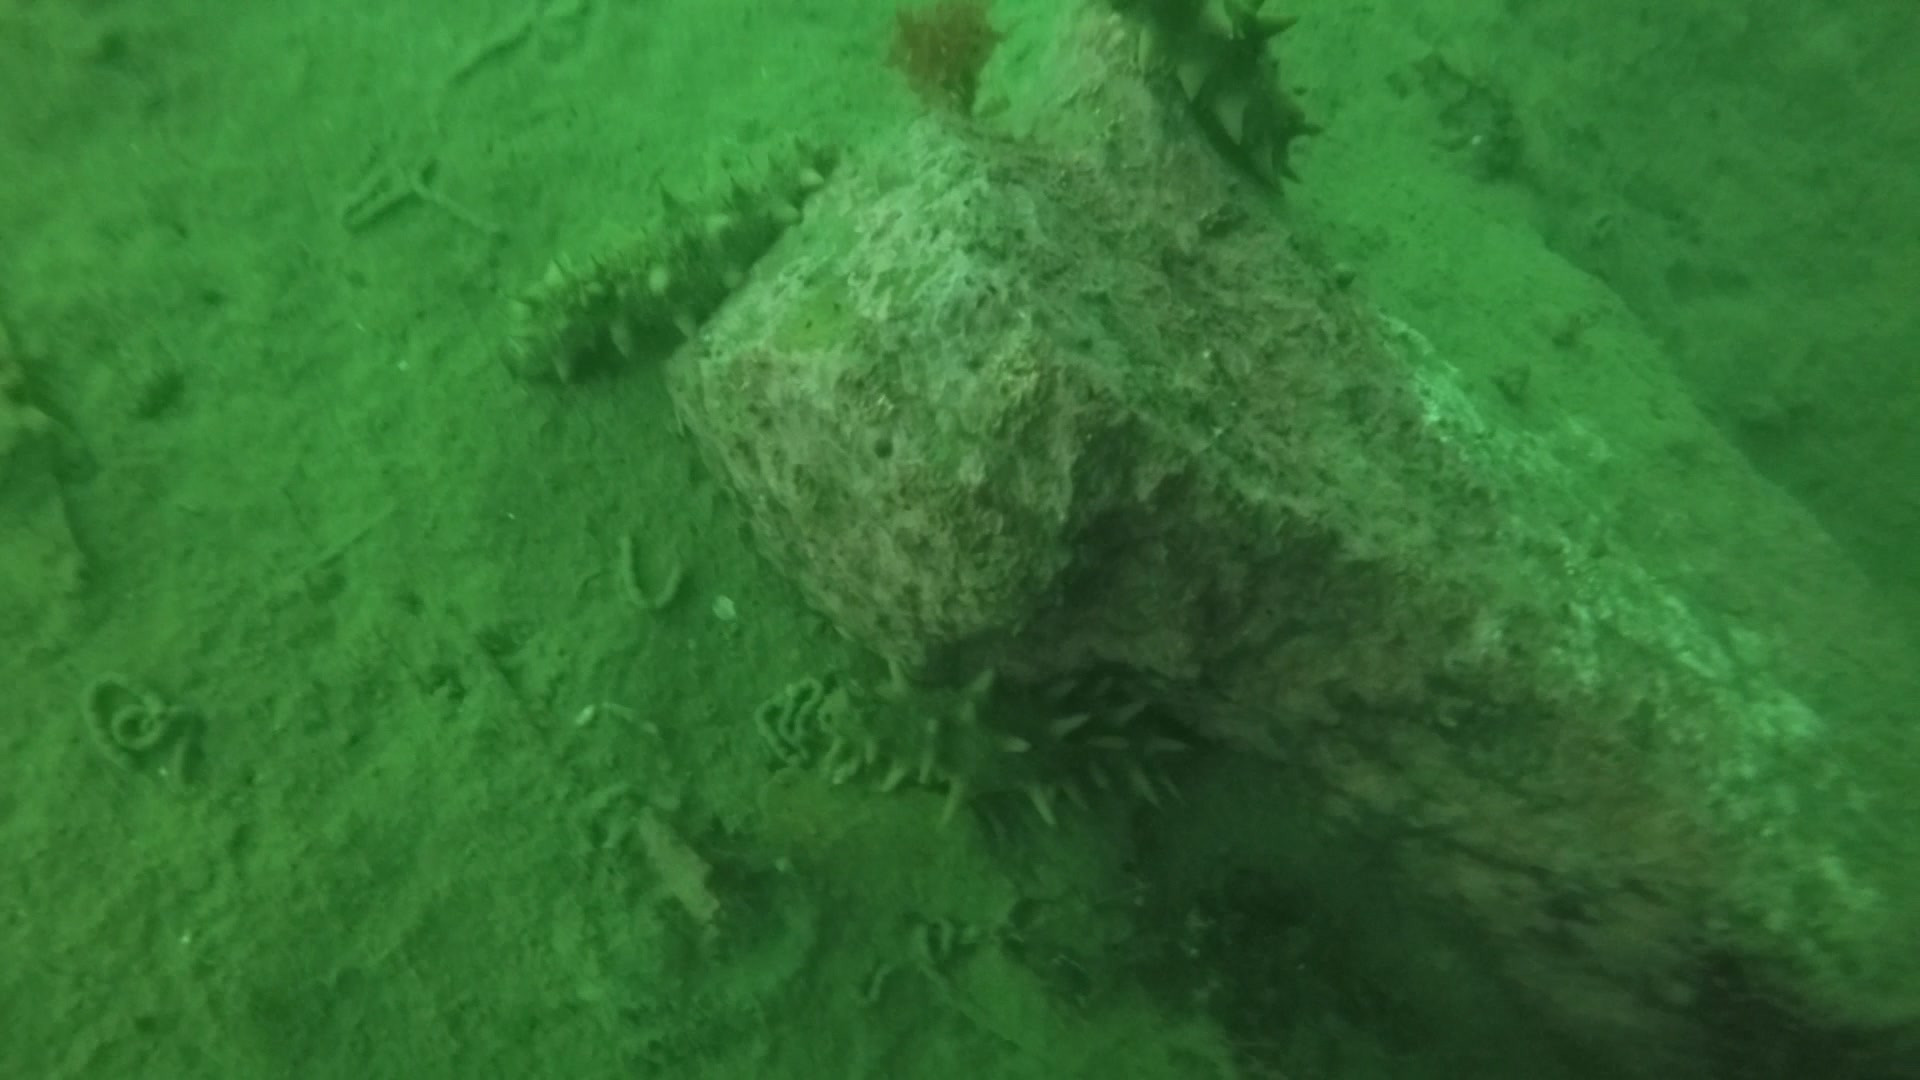}
\end{subfigure}
\caption{Sample images from UODD dataset containing underwater objects with complex backgrounds and varying visibility conditions.}
\label{fig:uodd_samples}
\end{figure}

%%%%%%%%%%%%%%%%%%%%%%%%%%%%%%%%%%%%%%%%%%%%%%%%%%%%%%%%%%%%%%%%%%%%%%%%%%%%%%%%%%%%
%%%%%%%%%%%%%%%%%%%%%%%%%%%%%%%%%%%%%%%%%%%%%%%%%%%%%%%%%%%%%%%%%%%%%%%%%%%%%%%%%%%%
\section{Computational Efficiency Analysis}

Our proposed framework demonstrates exceptional efficiency across multiple computational metrics. As shown in Table~\ref{tab:computational_overhead}, our method maintains practical deployment feasibility while delivering significant performance improvements.

\textbf{Zero-Parameter Design.} Our method maintains exactly 232.53M total parameters and 123.33M trainable parameters across all configurations, demonstrating complete parameter efficiency. PPR and NCM operate through feature space manipulations without introducing learnable parameters, while TSA leverages existing BERT encoder and projection layers from the baseline GLIP, ensuring no additional parameter overhead.

\textbf{Memory Efficiency.} The framework exhibits excellent memory efficiency, with cached memory increasing modestly from 3.09GB to 3.64GB (+18\%) when all modules are activated. Meanwhile, allocated memory remains almost constant (~1.95GB) across configurations, indicating stable runtime memory usage.

\textbf{Computational Efficiency.} FLOPs analysis confirms the lightweight nature of the proposed modules. PPR+NCM introduces only 1.3G additional FLOPs (+0.17\%), TSA adds 2.9G (+0.39\%), and the full framework incurs merely 4.2G additional FLOPs (+0.56\%) over the baseline. This reflects the efficiency of our prototype-based attention refinement compared to conventional attention mechanisms.

\textbf{Practical Implications.} The zero-parameter design enables seamless integration into existing architectures, while memory and computational costs are kept minimal. These advantages make our method suitable for real-world deployment scenarios, offering substantial gains in cross-domain detection performance with negligible overhead.

\begin{table*}[h]
\centering
\begin{tabular}{l|c|c|c|c|c}
\hline
\textbf{Method} & \textbf{Cached} & \textbf{Total} & \textbf{Trainable} & \textbf{Allocated} & \textbf{FLOPs} \\
 & \textbf{Memory (GB)} & \textbf{Params (M)} & \textbf{Params (M)} & \textbf{Memory (GB)} & \textbf{(G)} \\
\hline
Baseline & 3.09 & 232.53 & 123.33 & 1.95 & 743.9 \\
+PPR+NCM & 3.13 & 232.53 & 123.33 & 1.96 & 745.2 \\
+TSA & 3.53 & 232.53 & 123.33 & 1.95 & 746.8 \\
+PPR+NCM+TSA & 3.64 & 232.53 & 123.33 & 1.95 & 748.1 \\
\hline
\end{tabular}
\caption{Computational Overhead Analysis}
\label{tab:computational_overhead}
\end{table*}

\begin{figure*}[t]
    \centering
    \includegraphics[width=\linewidth]{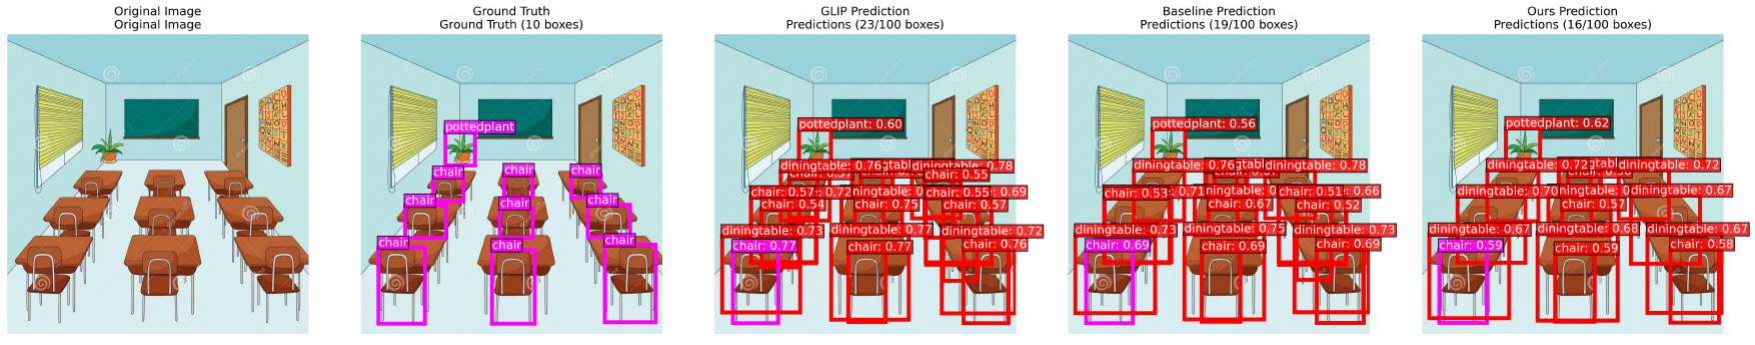}
    \vspace{0.2cm}
    
    \includegraphics[width=\linewidth]{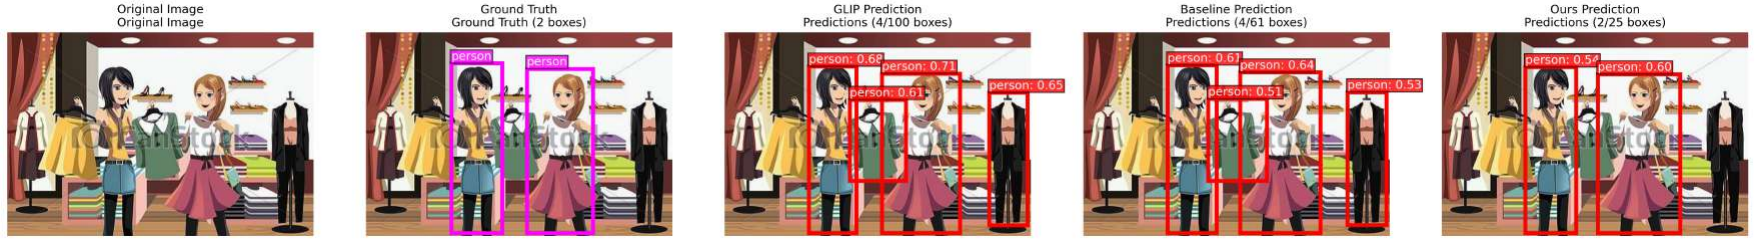}
    \vspace{0.2cm}
    
    \includegraphics[width=\linewidth]{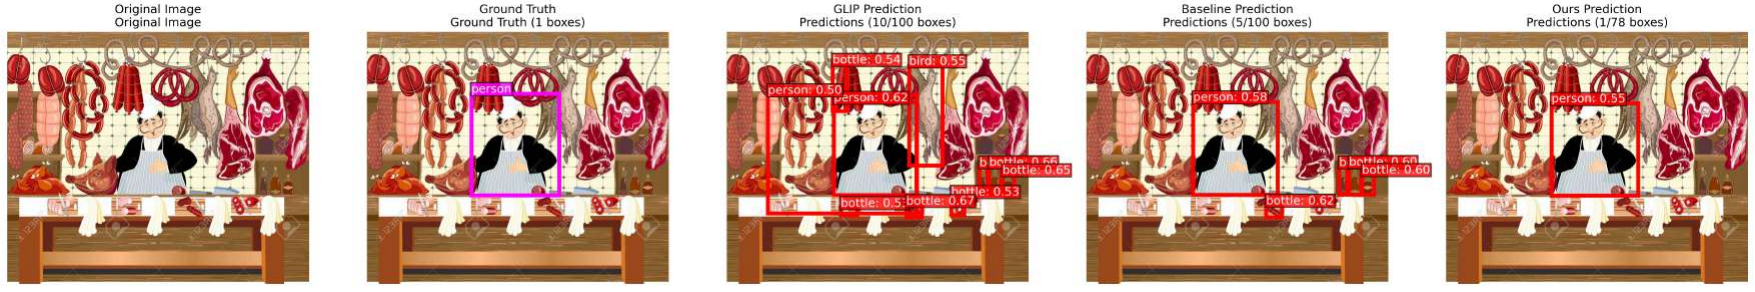}
    \vspace{0.2cm}
    
    \includegraphics[width=\linewidth]{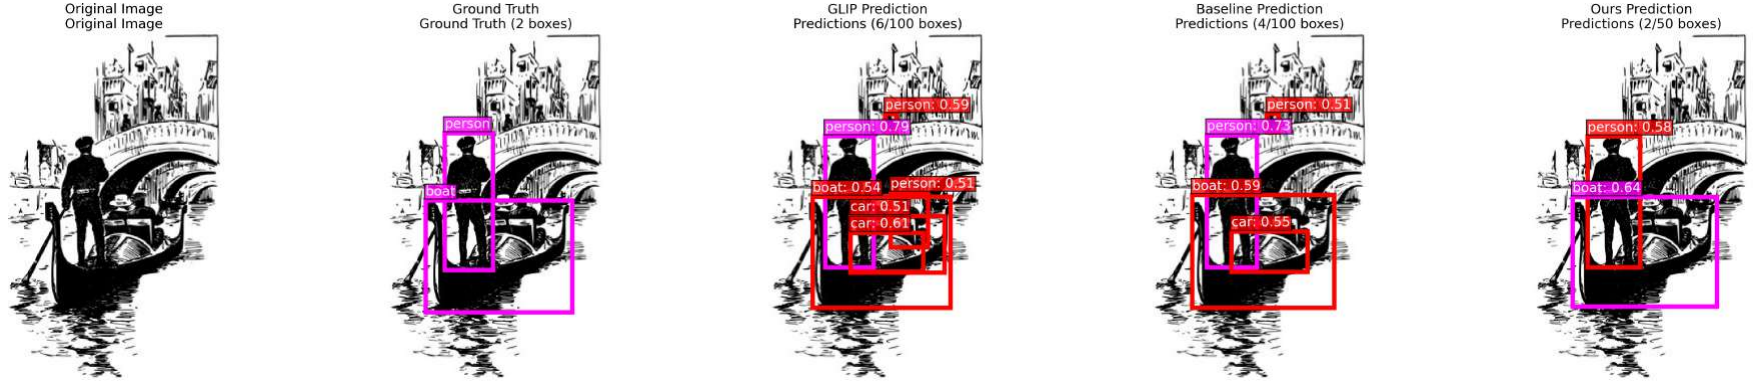}
    \vspace{0.2cm}
    
    \includegraphics[width=\linewidth]{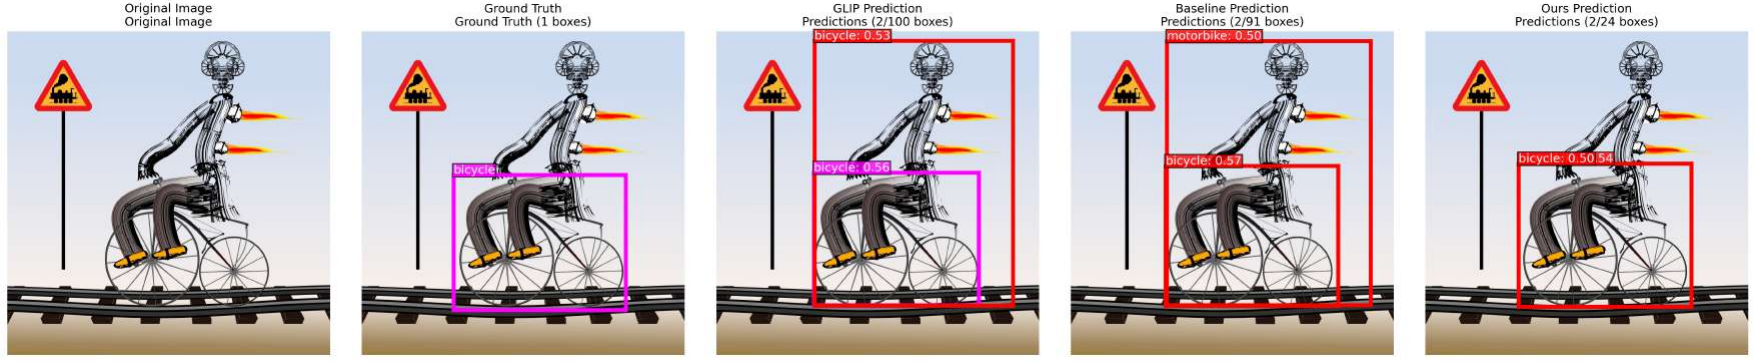}
    
    \caption{Comprehensive detection quality comparison across multiple test cases. Each row shows (from left to right): Original image, Ground truth annotations, GLIP predictions, Baseline predictions, and Our method predictions. Our approach consistently produces cleaner, more precise bounding boxes with significantly reduced false positives and better object-background separation across diverse scenarios and domains.}
    \label{fig:detection_quality_comparison}
\end{figure*}
%%%%%%%%%%%%%%%%%%%%%%%%%%%%%%%%%%%%%%%%%%%%%%%%%%%%%%%%%%%%%%%%%%%%%%%%%%%%%%%%%%%%
%%%%%%%%%%%%%%%%%%%%%%%%%%%%%%%%%%%%%%%%%%%%%%%%%%%%%%%%%%%%%%%%%%%%%%%%%%%%%%%%%%%%
\section{Detection Box Quality Analysis}

To provide comprehensive evidence of our method's superior detection quality, we present detailed visualizations comparing bounding box predictions across different approaches. Figure~\ref{fig:detection_quality_comparison} demonstrates our method's ability to generate precise, non-redundant detections while effectively suppressing background interference.

The visualizations reveal several key improvements:

\textbf{Precision Enhancement:} Our method consistently produces tighter, more accurate bounding boxes that closely align with ground truth annotations. The Positive Pattern Refinement module effectively guides attention toward object boundaries, resulting in more precise localization compared to baseline approaches that often generate loose or imprecise boxes.

\textbf{Redundancy Reduction:} Our approach generates cleaner, non-redundant predictions by suppressing multiple overlapping detections for the same object. This improvement stems from our Negative Context Modulation module, which enhances object-background distinctions and reduces false positive activations.

\textbf{Background Suppression:} The comparisons show superior background suppression capability, where our method effectively reduces false positives in background regions. Our Textual Semantic Alignment module strengthens semantic understanding of object-background relationships, addressing the common issue of misclassifying background regions as objects.

These qualitative results remain consistent across different target domains, supporting our quantitative findings and confirming that our center-periphery framework effectively addresses the Astigmatism problem in cross-domain few-shot detection scenarios.

%%%%%%%%%%%%%%%%%%%%%%%%%%%%%%%%%%%%%%%%%%%%%%%%%%%%%%%%%%%%%%%%%%%%%%%%%%%%%%%%%%%%
%%%%%%%%%%%%%%%%%%%%%%%%%%%%%%%%%%%%%%%%%%%%%%%%%%%%%%%%%%%%%%%%%%%%%%%%%%%%%%%%%%%%

\section{Background Text Design and Dataset Categories}

Our Negative Context Modulation module leverages carefully crafted background text descriptions to enhance object-background discrimination. This section provides detailed information about the background text design strategy and the specific categories for each evaluated dataset.

\subsubsection{Dataset Categories and Background Text Examples}

\paragraph{ArTaxOr Dataset}
\textbf{Target Categories:} 7 arthropod orders including Araneae (spiders), Coleoptera (beetles), Diptera (flies), Hemiptera (true bugs), Hymenoptera (bees, wasps, ants), Lepidoptera (butterflies, moths), and Odonata (dragonflies, damselflies).

\textbf{Representative Background Text Examples:}
\begin{itemize}
    \item \textit{Natural habitats:} "leaf surface", "tree bark", "plant stem", "forest floor", "meadow grass", "soil surface", "rock surface", "water surface"
    \item \textit{Direct negations:} "not Araneae", "not a spider", "not Coleoptera", "not a beetle", "not Diptera", "not a fly", "definitely not Hymenoptera", "absolutely not Lepidoptera"
    \item \textit{Species negations:} "area without spiders", "region with no beetles", "space lacking flies", "habitat devoid of bees and wasps", "environment free of butterflies or moths"
    \item \textit{Plant elements:} "green leaf", "plant texture", "flower", "twig", "branch", "grass", "tree trunk", "vegetation", "moss", "lichen"
    \item \textit{Contextual negations:} "empty leaf without insects", "bare tree bark with no spiders", "clean flower petals without butterflies", "undisturbed soil without beetles", "insect habitat currently unoccupied", "nectar source without pollinating insects"
    \item \textit{Natural environments:} "natural background", "habitat background", "ecological background", "wild background", "natural setting", "outdoor setting", "natural substrate"
\end{itemize}

\paragraph{CliPart1k Dataset}
\textbf{Target Categories:} 20 object classes including sheep, chair, boat, bottle, dining table, sofa, cow, motorbike, car, aeroplane, cat, train, person, bicycle, potted plant, bird, dog, bus, TV monitor, and horse.

\textbf{Representative Background Text Examples:}
\begin{itemize}
    \item \textit{Cartoon-specific elements:} "cartoon blank speech bubble", "clipart empty thought cloud", "illustrated vacant panel"
    \item \textit{Direct negations:} "not a sheep", "definitely not a chair", "absolutely not a boat"
    \item \textit{Environmental descriptions:} "empty cartoon theater", "vacant clipart stadium", "cartoon sky without objects"
    \item \textit{Stylistic backgrounds:} "dotted pattern background", "striped cartoon backdrop", "geometric mosaic background"
    \item \textit{Contextual negations:} "cartoon room without furniture or people", "clipart outdoor scene without vehicles or animals"
\end{itemize}

\textbf{Representative Background Text Examples:}
\begin{itemize}
    \item \textit{Land cover types:} "vegetation", "forest", "grassland", "agricultural field", "bare soil", "desert", "water body", "lake", "river", "coastline", "mountain", "urban area", "rural area"
    \item \textit{Direct negations:} "not airplane", "not airport", "not ship", "not harbor", "not bridge", "not dam", "definitely not golffield", "absolutely not stadium", "certainly not vehicle", "clearly not windmill"
    \item \textit{Infrastructure negations:} "area without buildings", "region with no vehicles", "space lacking transportation infrastructure", "terrain free of industrial structures", "landscape without recreational facilities"
    \item \textit{Satellite perspectives:} "satellite background", "aerial background", "remote sensing background", "earth surface background", "terrain background", "top-down perspective", "overhead view"
    \item \textit{Contextual negations:} "forested area without structures", "agricultural land without vehicles", "water body without ships", "open field without sports courts", "potential airport location but no airport present", "roadway without expressway service areas", "water area suitable for harbor but none exists"
    \item \textit{Natural landscapes:} "natural terrain", "undeveloped land", "pristine landscape", "uninhabited area", "natural coastline", "wilderness area", "unmodified terrain"
\end{itemize}

\paragraph{UODD Dataset}
\textbf{Target Categories:} 3 marine species including sea cucumber, sea urchin, and scallop.

\textbf{Representative Background Text Examples:}
\begin{itemize}
    \item \textit{Marine environments:} "sandy seafloor", "rocky ocean floor", "underwater terrain", "marine substrate"
    \item \textit{Species negations:} "not a sea cucumber", "definitely not a sea urchin", "certainly not a scallop"
    \item \textit{Habitat descriptions:} "area without sea cucumbers", "seafloor devoid of scallops", "marine environment without echinoderms"
    \item \textit{Water conditions:} "murky water", "clear water background", "turbid water", "suspended particles in water"
    \item \textit{Contextual negations:} "underwater habitat missing all target species", "seafloor with feeding trails but no sea cucumbers present"
\end{itemize}

\paragraph{NEU-DET Dataset}
\textbf{Target Categories:} 6 steel surface defect types including crazing, inclusion, patches, pitted surface, rolled-in scale, and scratches.

\textbf{Representative Background Text Examples:}
\begin{itemize}
    \item \textit{Surface quality:} "defect-free", "clean surface", "unblemished area", "standard surface", "flawless section"
    \item \textit{Defect negations:} "not crazing", "definitely not inclusion", "absolutely not patches", "certainly not pitted surface"
    \item \textit{Material descriptions:} "steel surface", "hot-rolled steel", "uniform texture", "metallic texture", "consistent grain pattern"
    \item \textit{Quality indicators:} "standard production quality", "within-spec finish", "quality control passed surface"
    \item \textit{Contextual negations:} "uniform steel surface without crazing", "smooth metal with no inclusions"
\end{itemize}

\paragraph{FISH Dataset}
\textbf{Target Categories:} Multiple fish species in underwater environments.

\textbf{Representative Background Text Examples:}
\begin{itemize}
    \item \textit{Aquatic environments:} "underwater background", "marine background", "open water", "coral reef", "seagrass bed"
    \item \textit{Fish negations:} "not a fish", "definitely not a fish", "area without fish", "completely fish-free zone"
    \item \textit{Water conditions:} "clear water", "murky water", "shallow water", "deep water", "sunlit water"
    \item \textit{Habitat descriptions:} "coral reef without fish", "seagrass bed with no fish", "underwater cave devoid of fish"
    \item \textit{Contextual negations:} "underwater habitat that typically contains fish but currently empty", "natural fish shelter without occupants"
\end{itemize}

\section{Background Text Design Principles}

Our background text design follows key principles to maximize the effectiveness of the Negative Context Modulation module:

\textbf{Domain-Specific Adaptation:} Background text is tailored to each dataset's visual domain. For cartoon imagery (CliPart1k), we emphasize artistic elements; for industrial applications (NEU-DET), we focus on manufacturing contexts; for marine environments (UODD, FISH), we incorporate aquatic terminology; for biological detection (ArTaxOr), we utilize ecological and natural habitat descriptions; for remote sensing imagery (DIOR), we employ geographical and infrastructure-related terminology.

\textbf{Multi-Level Negation Strategy:} We employ various negation approaches including direct class negations ("not a sheep"), alternative phrasings ("area without sheep"), and contextual negations ("cartoon room without furniture"). This ensures robust background-foreground discrimination across different linguistic formulations.

\textbf{Environmental Context Integration:} Background descriptions incorporate domain-relevant environmental context, helping the model understand typical object settings and enhancing semantic understanding of object-background relationships.

\textbf{Hierarchical Coverage:} Text descriptions range from general background terms to specific contextual negations, allowing the model to learn background representations at multiple abstraction levels. Each dataset includes hundreds of variations to ensure comprehensive coverage and prevent overfitting.

\textbf{Adaptive Text Selection via TSA:} Given the extensive background text vocabulary, our Textual Semantic Alignment (TSA) module employs a softmax function with temperature scaling to dynamically select the most semantically relevant background descriptions for each image. The temperature coefficient controls the sharpness of the attention distribution, allowing the model to focus more on background texts that are semantically similar to the current image features. This adaptive selection mechanism ensures that only the most contextually appropriate negative descriptions are emphasized during training, improving the efficiency and effectiveness of background-foreground discrimination.

The effectiveness of this design is demonstrated through our attention distance analysis and detection quality improvements, confirming that well-crafted negative context descriptions with adaptive selection significantly enhance cross-domain few-shot detection performance.

%%%%%%%%%%%%%%%%%%%%%%%%%%%%%%%%%%%%%%%%%%%%%%%%%%%%%%%%%%%%%%%%%%%%%%%%%%%%%%%%%%%%
%%%%%%%%%%%%%%%%%%%%%%%%%%%%%%%%%%%%%%%%%%%%%%%%%%%%%%%%%%%%%%%%%%%%%%%%%%%%%%%%%%%%

%%%%%%%%%%%%%%%%%%%%%%%%%%%%%%%%%%%%%%%%%%%%%%%%%%%%%%%%%%%%%%%%%%%%%%%%%%%%%%%%%%%%
%%%%%%%%%%%%%%%%%%%%%%%%%%%%%%%%%%%%%%%%%%%%%%%%%%%%%%%%%%%%%%%%%%%%%%%%%%%%%%%%%%%%
